# Supplementary material for: Enhancing Visual Interpretability and Explainability in Functional Survival Trees and Forests
Source: arXiv:2504.18498 source file (2025-04-25)
Supplement: Supplementary file 1 [file appendix.tex]

\section{Appendix}
\subsection*{Simulation study for $N=200$}
\begin{figure*}[h!]
    \centering
    \includegraphics[width=0.8\linewidth]{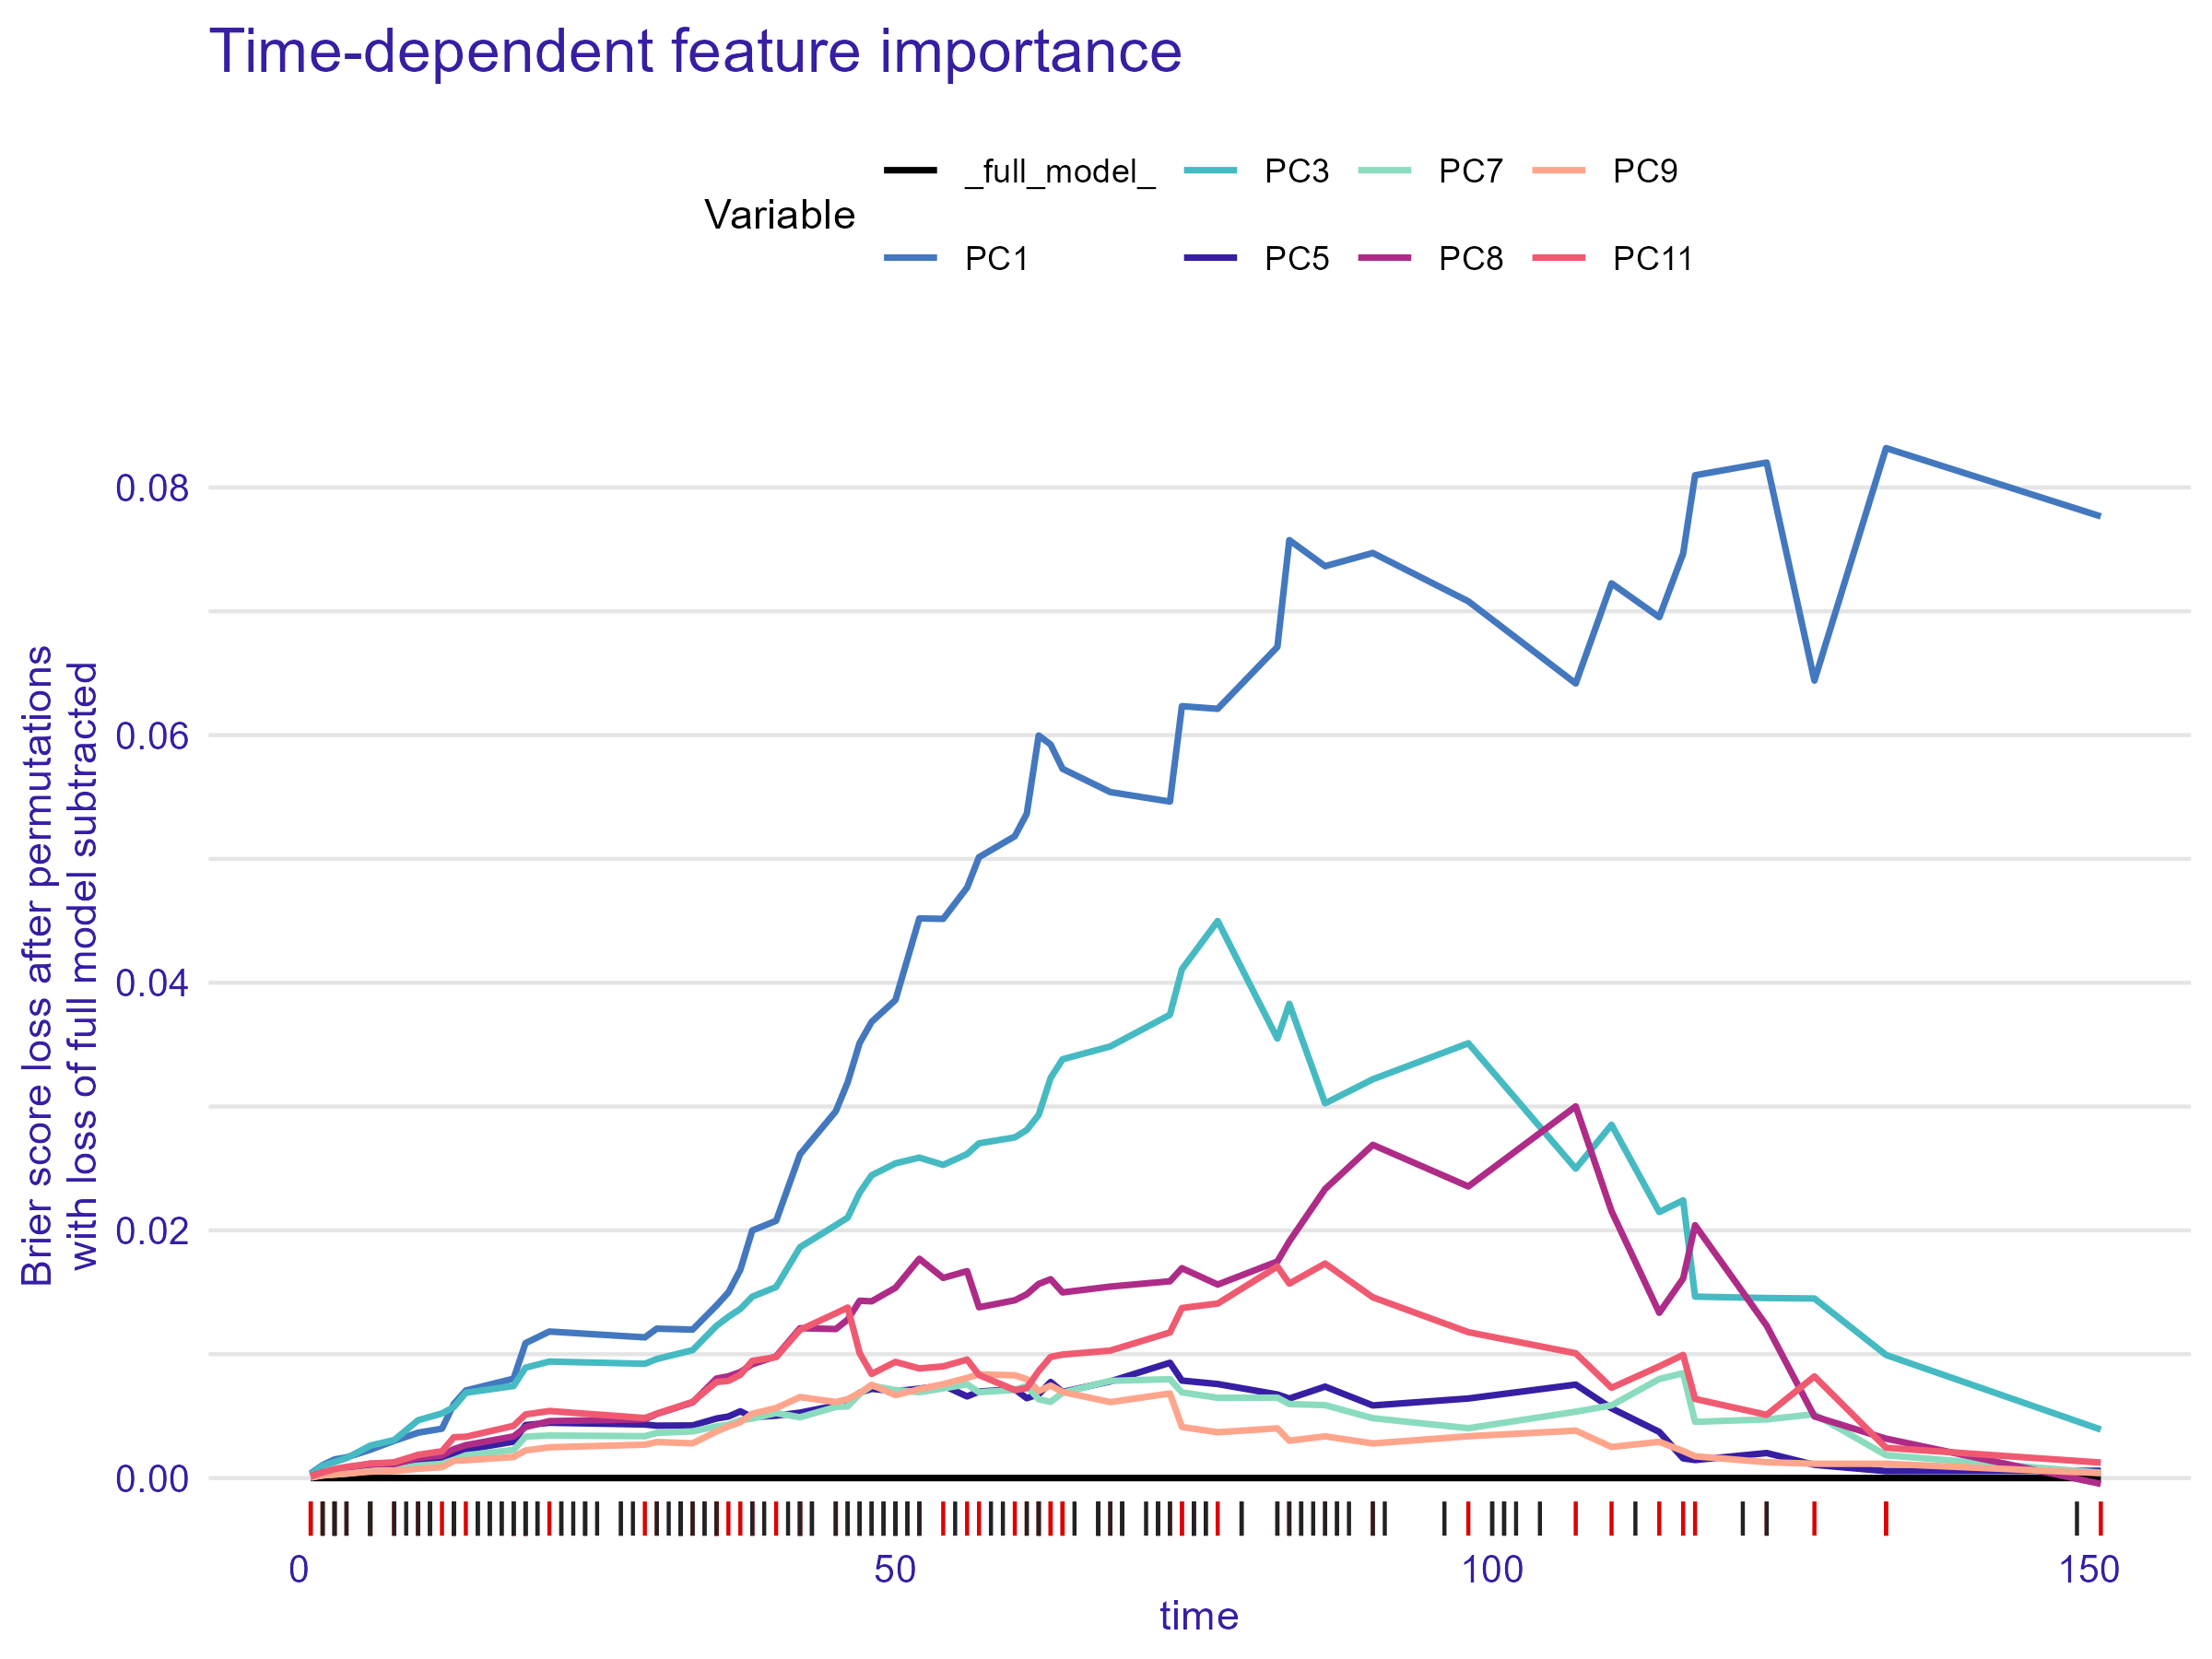}
    \includegraphics[width=0.8\linewidth]{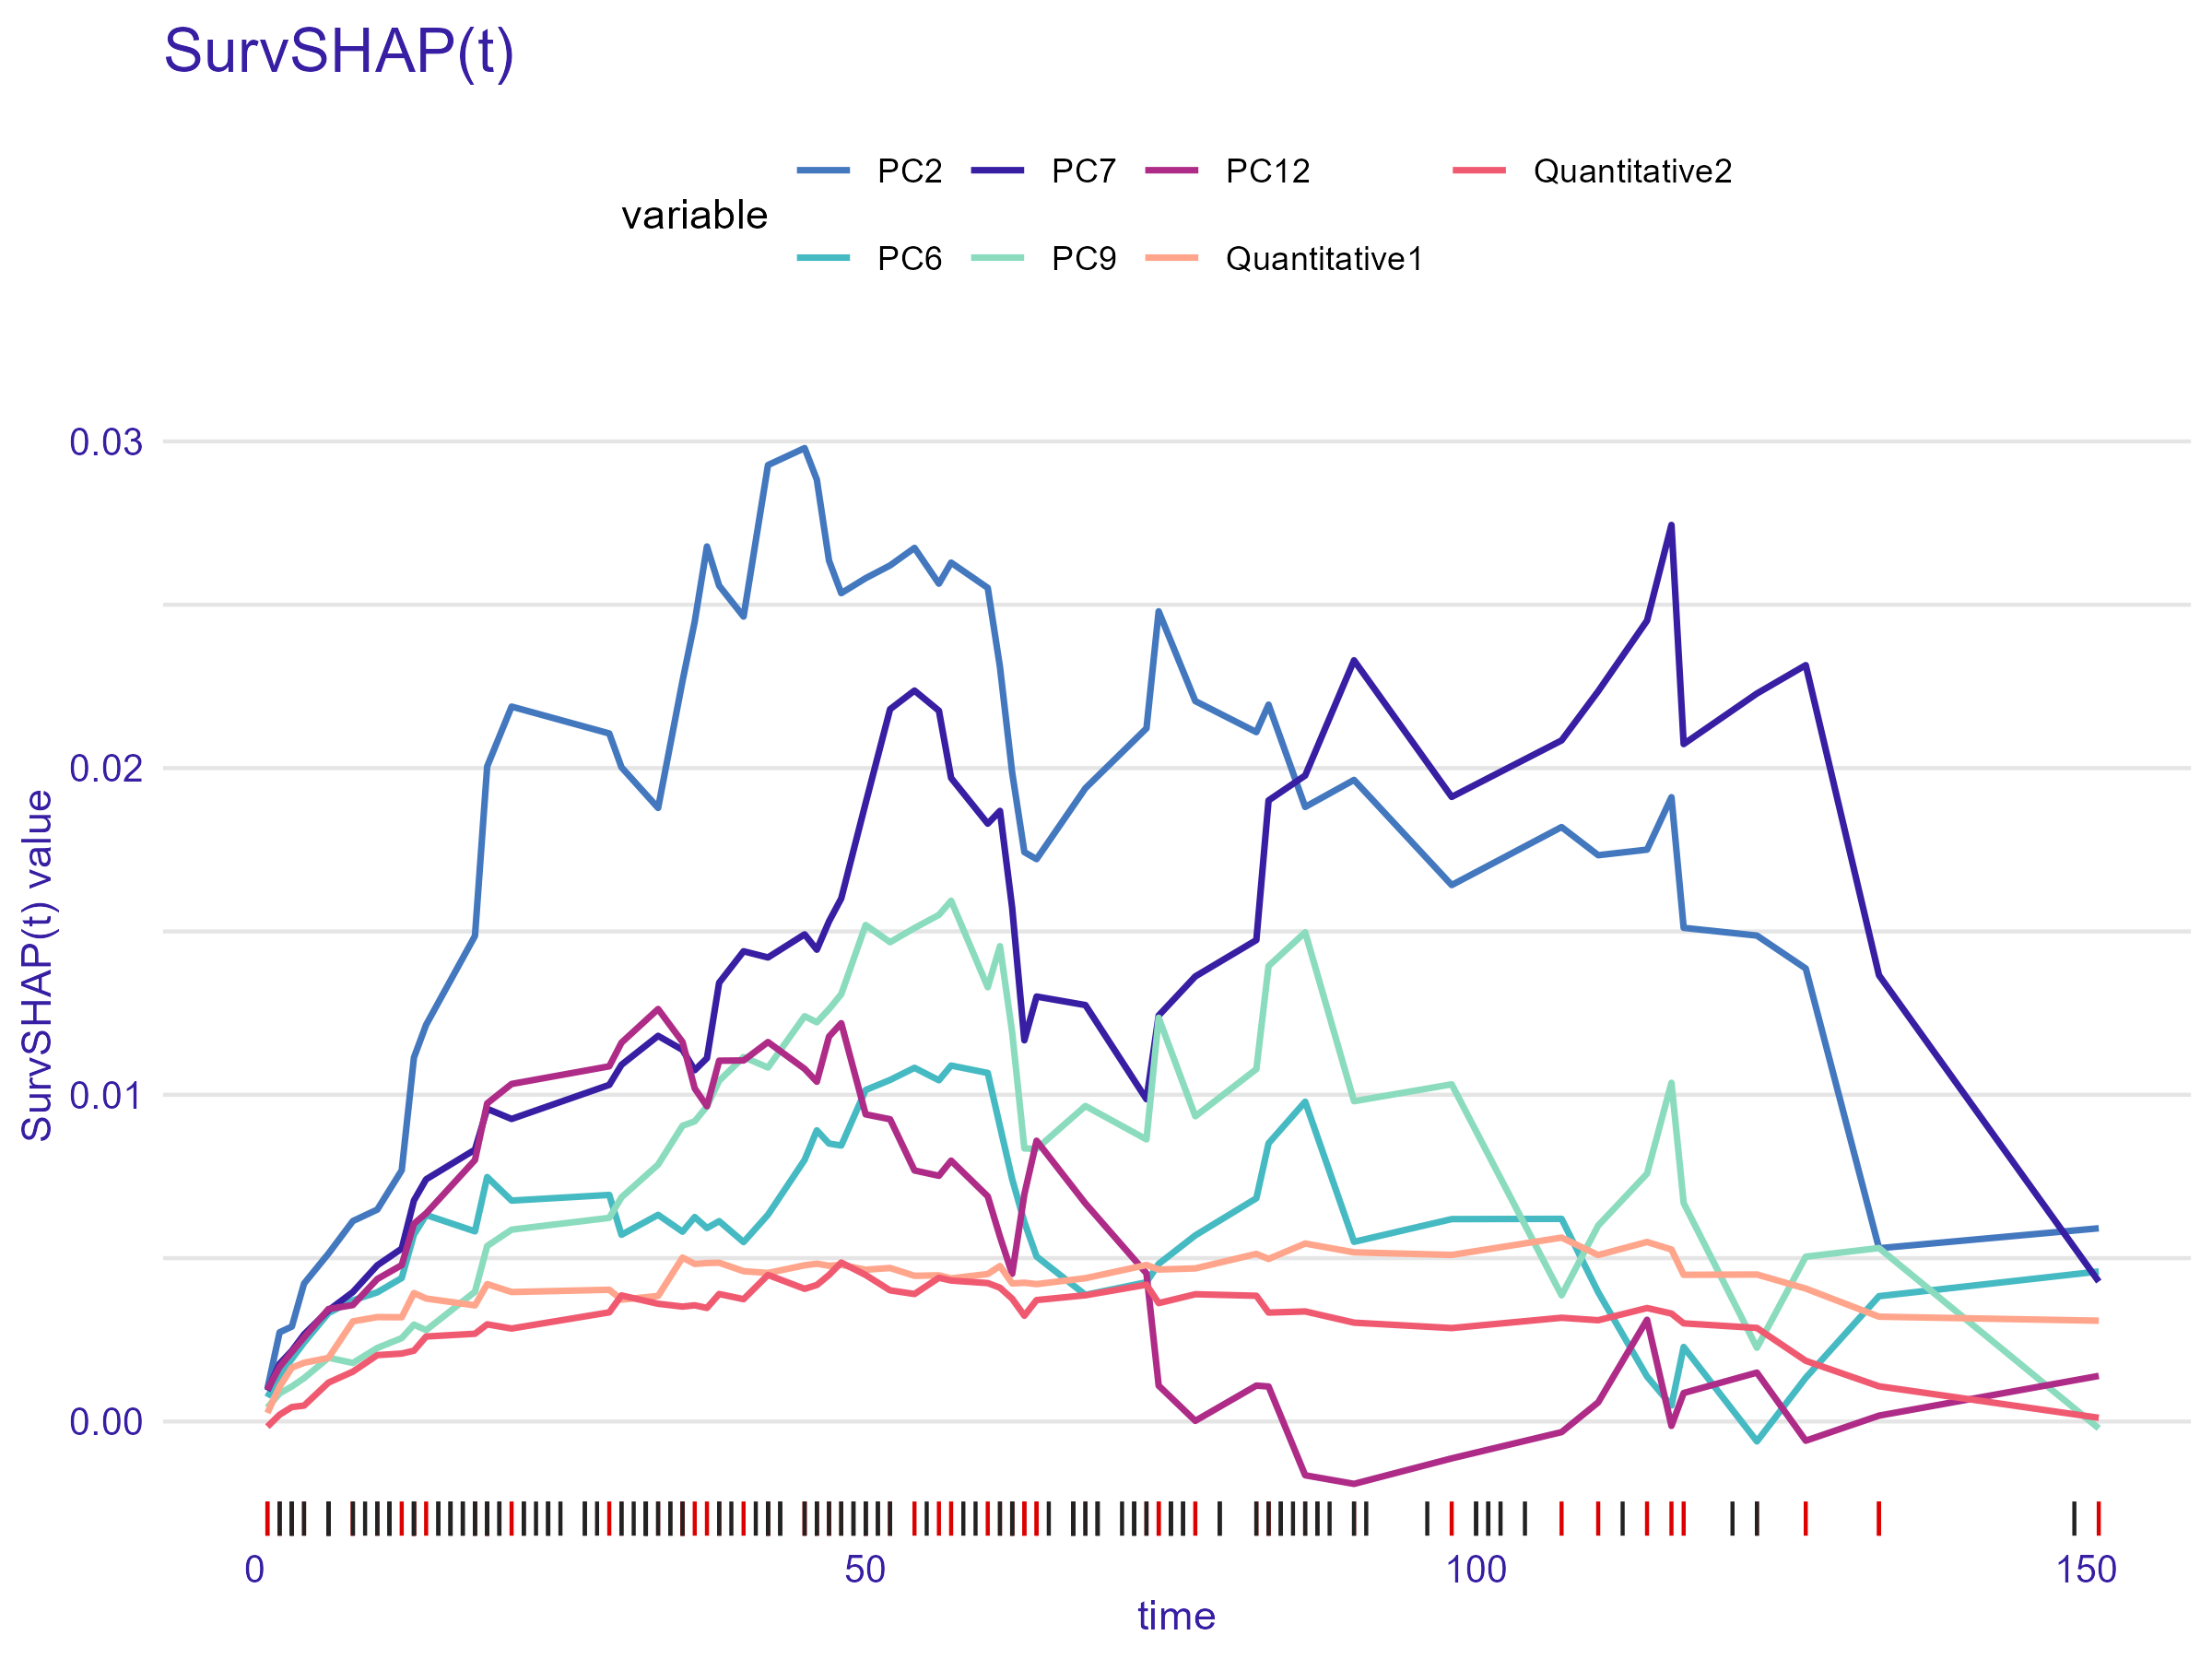}
    \caption{Caption}
    \label{fig:enter-label}
\end{figure*}

\begin{table*}
\Large
\centering
\begin{minipage}{0.54\textwidth}
\centering
 % Aumenta l'altezza delle righe
\setlength{\tabcolsep}{19pt} % Aumenta la spaziatura tra le colonne
\resizebox{\textwidth}{!}{ % Adatta la tabella alla larghezza della pagina
\begin{tabular}{c|cc|c|c} 
\hline
\hline
\multicolumn{5}{c}{\textbf{Global Explainability for PC1}} \\  
\hline
\hline
\multirow{2}{*}{\([t_\alpha,t_\beta]\)} & \multicolumn{2}{c|}{\(PFI_1(t)\)} & \multirow{2}{*}{\(MTSD_{t_\alpha,t_\beta}^{1}\)} &\multirow{2}{*} {\(MTNSD_{t_\alpha,t_\beta}^{1}\)} \\ \cline{2-3}
                        & \(PFI_1(t_\alpha)\) & \(PFI_1(t_\beta)\) &  &  \\ 
\hline
[4,6]                    & 0.00185283 & 0.00245758 & $-5.38 \times 10^{-6}$ & $-2.69 \times 10^{-6}$ \\ \hline
[6,8]                    & 0.00245758 & 0.00316047 & $1.49 \times 10^{-5}$  & $7.45 \times 10^{-6}$  \\ \hline
[8,10]                   & 0.00316047 & 0.00355074 & $6.46 \times 10^{-5}$  & $3.23 \times 10^{-5}$  \\ \hline
[10,12]                  & 0.00355074 & 0.00394254 & $-3.04 \times 10^{-4}$ & $-1.52 \times 10^{-4}$ \\ \hline
[14,18]                  & 0.00679740 & 0.00730410 & $-1.65 \times 10^{-3}$ & $-4.12 \times 10^{-4}$ \\ \hline
[19,21]                  & 0.00991108 & 0.01144837 & $4.16 \times 10^{-4}$  & $2.08 \times 10^{-4}$  \\ \hline
[21,29]                  & 0.01144837 & 0.01098038 & $3.05 \times 10^{-3}$  & $3.82 \times 10^{-4}$  \\ \hline
[30,33]                  & 0.01195368 & 0.01174326 & $-1.03 \times 10^{-3}$ & $-3.43 \times 10^{-4}$ \\ \hline
[33,35]                  & 0.01174326 & 0.01404944 & $-2.22 \times 10^{-4}$ & $-1.11 \times 10^{-4}$ \\ \hline
[38,40]                  & 0.02025410 & 0.02124029 & $-1.14 \times 10^{-4}$ & $-5.70 \times 10^{-5}$ \\ \hline
[40,42]                  & 0.02124029 & 0.02717545 & $-1.94 \times 10^{-4}$ & $-9.69 \times 10^{-5}$ \\ \hline
[42,45]                  & 0.02717545 & 0.03056935 & $7.71 \times 10^{-4}$  & $2.57 \times 10^{-4}$  \\ \hline
[48,50]                  & 0.03657040 & 0.03724537 & $-1.91 \times 10^{-4}$ & $-9.53 \times 10^{-5}$ \\ \hline
[50,52]                  & 0.03724537 & 0.04120939 & $4.77 \times 10^{-4}$  & $2.38 \times 10^{-4}$  \\ \hline
[52,54]                  & 0.04120939 & 0.04068467 & $-3.00 \times 10^{-4}$ & $-1.50 \times 10^{-4}$ \\ \hline
[54,56]                  & 0.04068467 & 0.04340819 & $-3.17 \times 10^{-4}$ & $-1.58 \times 10^{-4}$ \\ \hline
[57,60]                  & 0.04641078 & 0.04826712 & $-2.23 \times 10^{-4}$ & $-7.42 \times 10^{-5}$ \\ \hline
[64,68]                  & 0.05685593 & 0.05357206 & $2.83 \times 10^{-4}$  & $7.09 \times 10^{-5}$  \\ \hline
[68,73]                  & 0.05357206 & 0.05410605 & $-1.12 \times 10^{-2}$ & $-2.24 \times 10^{-3}$ \\ \hline
[74,77]                  & 0.06068427 & 0.06309772 & $3.53 \times 10^{-3}$  & $1.18 \times 10^{-3}$  \\ \hline
[77,82]                  & 0.06309772 & 0.06709227 & $-1.42 \times 10^{-2}$ & $-2.84 \times 10^{-3}$ \\ \hline
[83,86]                  & 0.07438620 & 0.07298383 & $4.72 \times 10^{-3}$  & $1.57 \times 10^{-3}$  \\ \hline
[86,90]                  & 0.07298383 & 0.07278383 & $-2.83 \times 10^{-3}$ & $-7.07 \times 10^{-4}$ \\ \hline
[90,98]                  & 0.07278383 & 0.06751300 & $1.09 \times 10^{-2}$  & $1.37 \times 10^{-3}$  \\ \hline
[98,107]                 & 0.06751300 & 0.06186418 & $-2.58 \times 10^{-2}$ & $-2.87 \times 10^{-3}$ \\ \hline
[107,110]                & 0.06186418 & 0.06943421 & $6.17 \times 10^{-4}$  & $2.06 \times 10^{-4}$  \\ \hline
[110,114]                & 0.06943421 & 0.06965263 & $5.69 \times 10^{-4}$  & $1.42 \times 10^{-4}$  \\ \hline
[114,116]                & 0.06965263 & 0.07486795 & $-1.20 \times 10^{-3}$ & $-6.01 \times 10^{-4}$ \\ \hline
[117,123]                & 0.08150482 & 0.07812225 & $2.70 \times 10^{-2}$  & $4.51 \times 10^{-3}$  \\ \hline
[123,127]                & 0.07812225 & 0.06493811 & $-2.77 \times 10^{-3}$ & $-6.94 \times 10^{-4}$ \\ \hline
[127,133]                & 0.06493811 & 0.07349230 & $-1.54 \times 10^{-2}$ & $-2.57 \times 10^{-3}$ \\ \hline
[133,151]                & 0.07349230 & 0.07439249 & $3.94 \times 10^{-1}$  & $2.19 \times 10^{-2}$  \\ \hline \hline
\end{tabular}
}
\caption{44}
\label{tabella_divisa}
\end{minipage} \vfill
\vspace{5mm}
\begin{minipage}{0.68\textwidth}
\centering
\includegraphics[width=\linewidth]{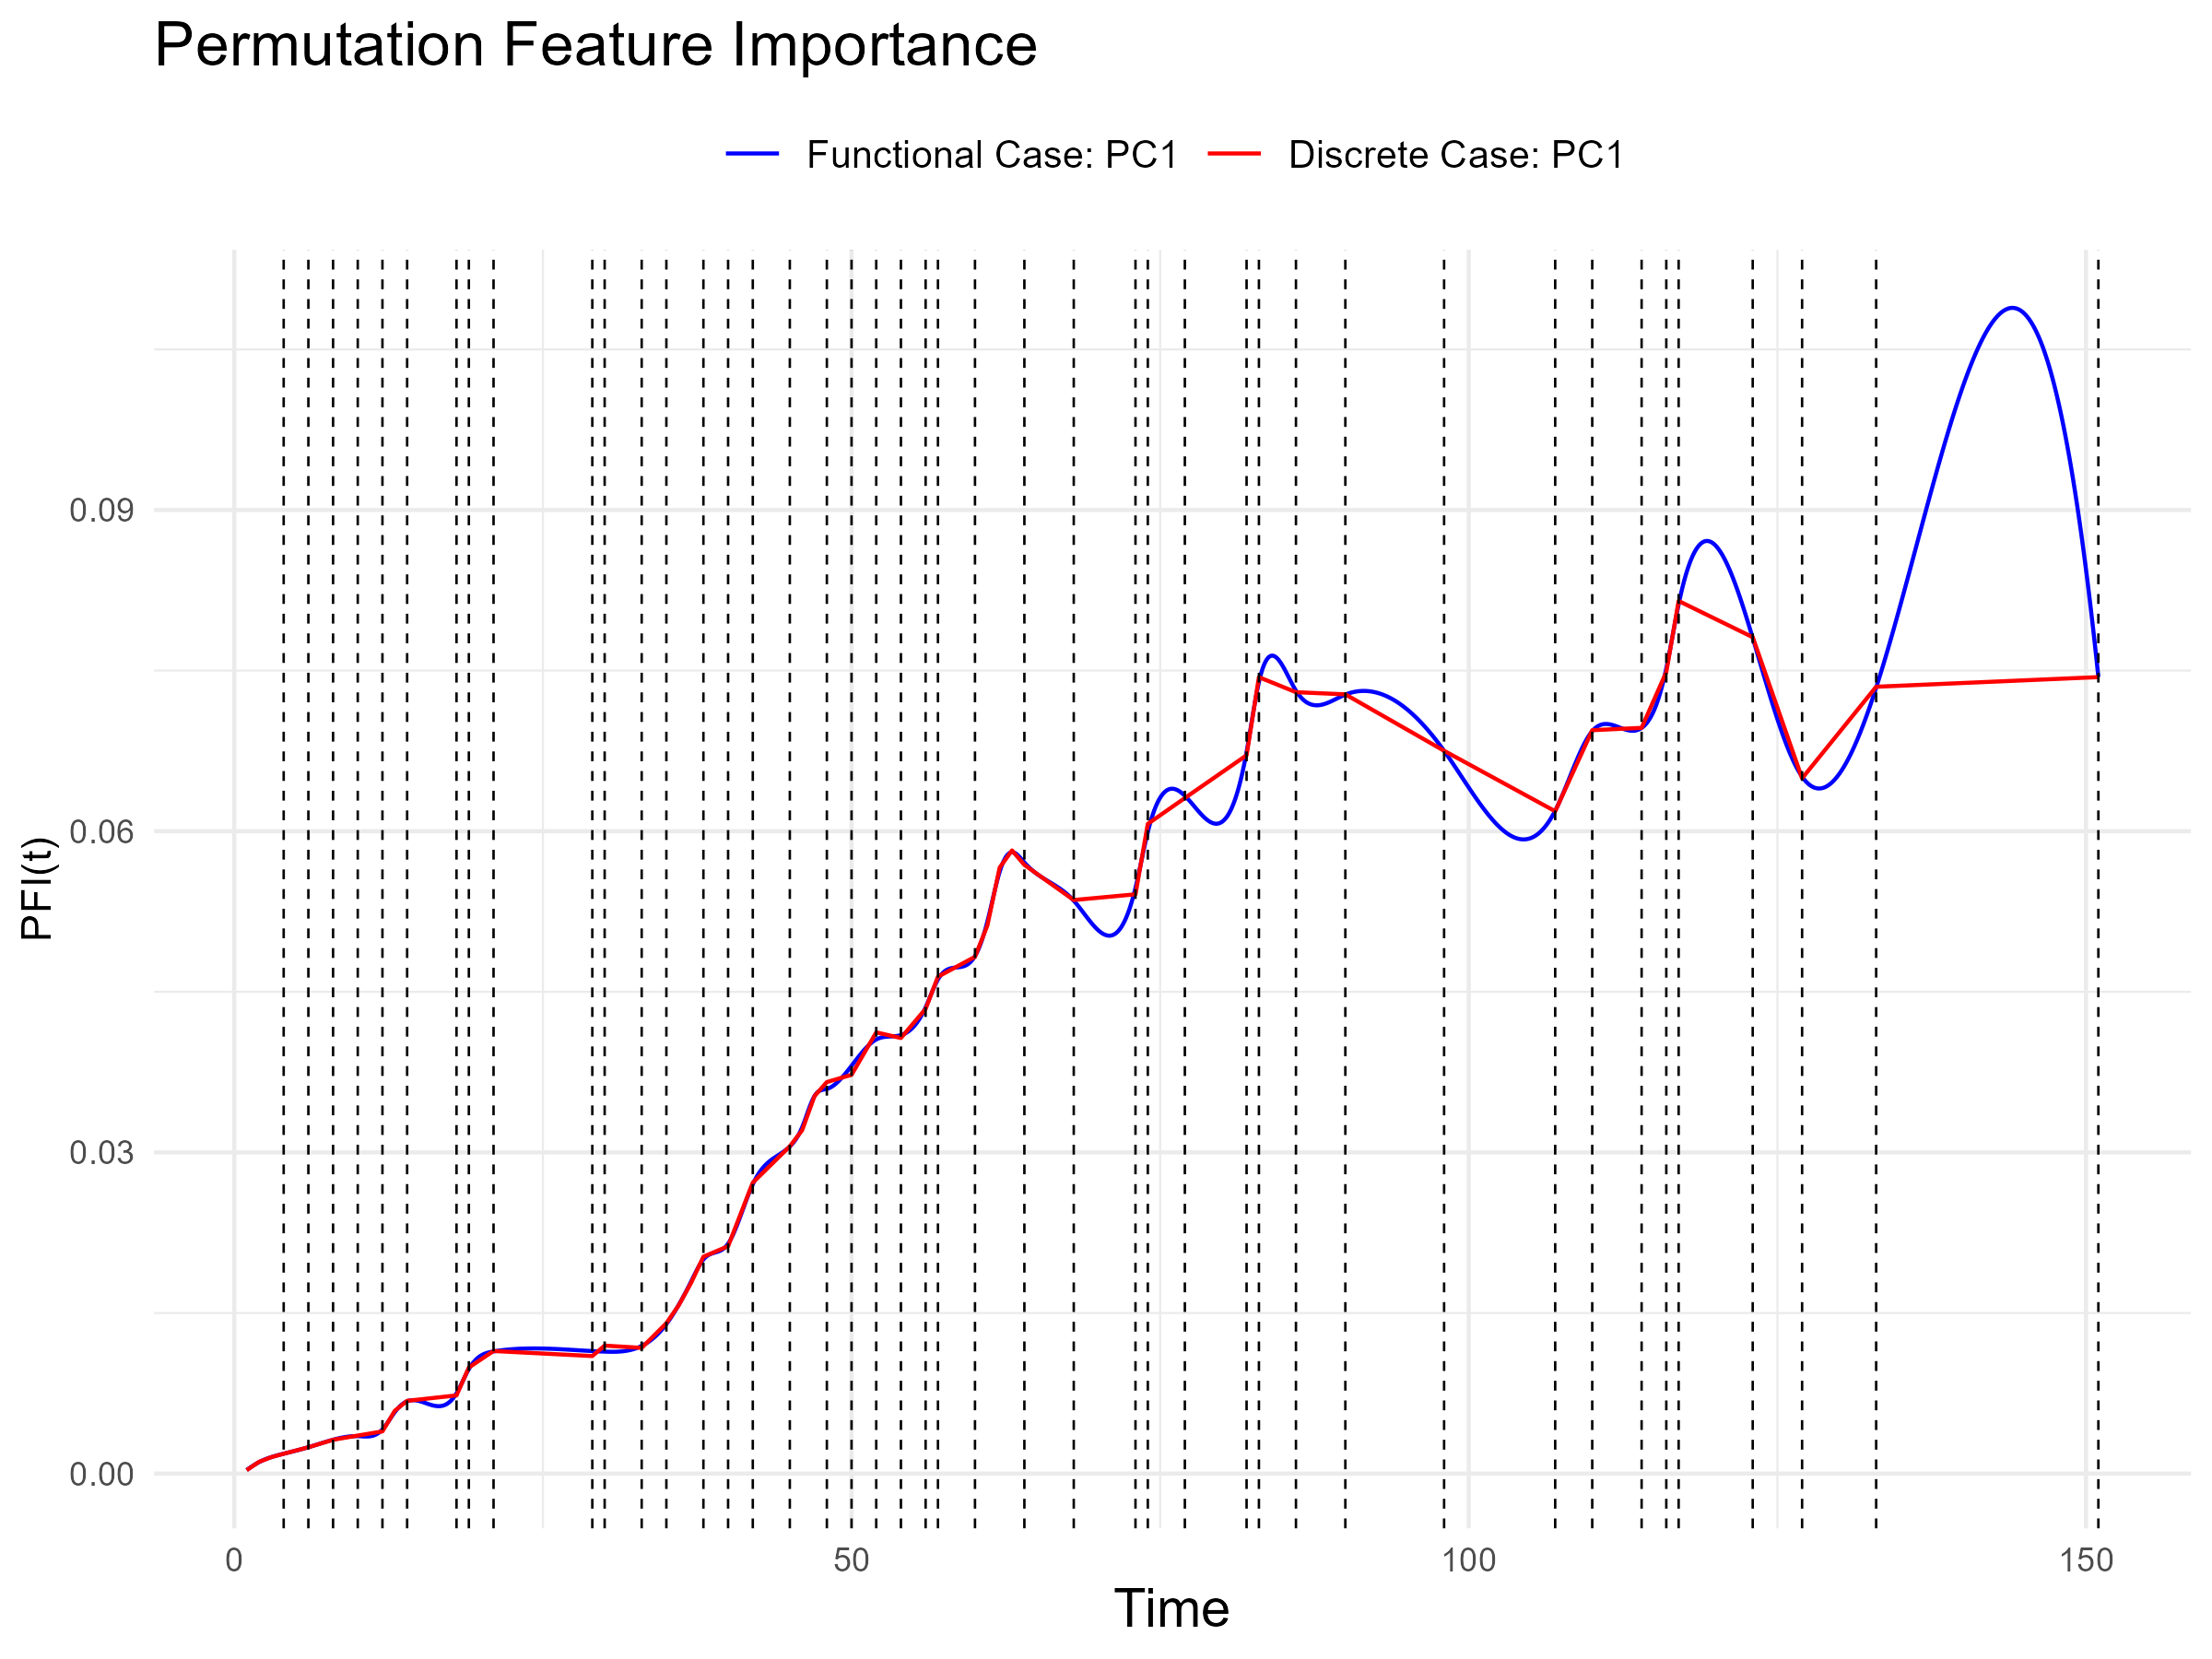}
\captionof{figure}{Descrizione dell'immagine.}
\label{fig:your_image}
\end{minipage}
\end{table*}  

\begin{table*}
\Large
\centering
\begin{minipage}{0.54\textwidth}
\centering
 % Aumenta l'altezza delle righe
\setlength{\tabcolsep}{19pt} % Aumenta la spaziatura tra le colonne
\resizebox{\textwidth}{!}{ % Adatta la tabella alla larghezza della pagina
\begin{tabular}{c|cc|c|c} 
\hline
\hline
\multicolumn{5}{c}{\textbf{Local Explainability for PC2 for $2$th unit}} \\  
\hline
\hline
\multirow{2}{*}{\([t_\alpha,t_\beta]\)} & \multicolumn{2}{c|}{\(\phi^*_t(\bm{w_*},2)\)} & \multirow{2}{*}{\(TSD_{t_\alpha,t_\beta}^{22}\)} &\multirow{2}{*} {\(TNSD_{t_\alpha,t_\beta}^{22}\)} \\ \cline{2-3}
                        & \(\phi^*_{t_\alpha}(\bm{w_*},2)\) & \(\phi^*_{t_\beta}(\bm{w_*},2)\) &  &  \\ 
\hline
[4,6]                    & 0.004221 & 0.005140   & $2.56 \times 10^{-5}$  & $7.82 \times 10^{-6}$  \\ \hline
[6,8]                    & 0.005140 & 0.006136   & $3.69 \times 10^{-5}$  & $1.84 \times 10^{-5}$  \\ \hline
[8,10]                   & 0.006136 & 0.006486   & $-1.92 \times 10^{-4}$ & $-9.60 \times 10^{-5}$ \\ \hline
[10,12]                  & 0.006486 & 0.007689   & $1.52 \times 10^{-4}$  & $7.61 \times 10^{-5}$  \\ \hline
[14,18]                  & 0.012143 & 0.014865   & $-3.68 \times 10^{-4}$ & $-9.20 \times 10^{-5}$ \\ \hline
[19,21]                  & 0.020052 & 0.021882   & $-2.66 \times 10^{-4}$ & $-1.33 \times 10^{-4}$ \\ \hline
[21,29]                  & 0.021882 & 0.021060   & $9.31 \times 10^{-3}$  & $1.16 \times 10^{-3}$  \\ \hline
[30,33]                  & 0.020025 & 0.018780   & $-8.92 \times 10^{-4}$ & $-2.97 \times 10^{-4}$ \\ \hline
[33,35]                  & 0.018780 & 0.022667   & $-1.86 \times 10^{-4}$ & $-9.31 \times 10^{-5}$ \\ \hline
[38,40]                  & 0.025583 & 0.024638   & $3.55 \times 10^{-4}$  & $1.78 \times 10^{-4}$  \\ \hline
[40,42]                  & 0.024638 & 0.029275   & $3.62 \times 10^{-5}$  & $1.81 \times 10^{-5}$  \\ \hline
[42,45]                  & 0.029275 & 0.029794   & $1.37 \times 10^{-3}$  & $4.56 \times 10^{-4}$  \\ \hline
[48,50]                  & 0.025354 & 0.025813   & $-2.62 \times 10^{-4}$ & $-1.31 \times 10^{-4}$ \\ \hline
[50,52]                  & 0.025813 & 0.026203   & $-1.76 \times 10^{-4}$ & $-8.79 \times 10^{-5}$ \\ \hline
[52,54]                  & 0.026204 & 0.026740   & $1.21 \times 10^{-4}$  & $7.46 \times 10^{-5}$  \\ \hline
[54,56]                  & 0.026740 & 0.025645   & $-5.77 \times 10^{-7}$ & $-2.89 \times 10^{-7}$ \\ \hline
[57,60]                  & 0.026289 & 0.025516   & $1.01 \times 10^{-3}$  & $3.37 \times 10^{-4}$  \\ \hline
[64,68]                  & 0.017213 & 0.019385   & $-1.75 \times 10^{-3}$ & $-4.36 \times 10^{-4}$ \\ \hline
[68,73]                  & 0.019385 & 0.021216   & $2.19 \times 10^{-3}$  & $4.39 \times 10^{-4}$  \\ \hline
[74,77]                  & 0.024798 & 0.022050   & $-3.46 \times 10^{-4}$ & $-1.15 \times 10^{-4}$ \\ \hline
[77,82]                  & 0.022050 & 0.021102   & $-1.47 \times 10^{-3}$ & $-2.94 \times 10^{-4}$ \\ \hline
[83,86]                  & 0.021942 & 0.018810   & $9.79 \times 10^{-4}$  & $3.26 \times 10^{-4}$  \\ \hline
[86,90]                  & 0.018810 & 0.019638   & $-1.07 \times 10^{-3}$ & $-2.67 \times 10^{-4}$ \\ \hline
[90,98]                  & 0.019638 & 0.016420   & $2.50 \times 10^{-3}$  & $3.12 \times 10^{-4}$  \\ \hline
[98,107]                 & 0.016420 & 0.018195   & $-1.03 \times 10^{-3}$ & $-1.15 \times 10^{-4}$ \\ \hline
[107,110]                & 0.018195 & 0.017333   & $1.21 \times 10^{-4}$  & $4.04 \times 10^{-5}$  \\ \hline
[110,114]                & 0.017333 & 0.017504   & $-2.77 \times 10^{-4}$ & $-6.93 \times 10^{-5}$ \\ \hline
[114,116]                & 0.017504 & 0.019109   & $-2.61 \times 10^{-4}$ & $-1.30 \times 10^{-4}$ \\ \hline
[117,123]                & 0.015110 & 0.014873   & $-3.72 \times 10^{-3}$ & $-6.21 \times 10^{-4}$ \\ \hline
[123,127]                & 0.014873 & 0.013865   & $1.29 \times 10^{-3}$  & $3.22 \times 10^{-4}$  \\ \hline
[127,133]                & 0.013865 & 0.005303   & $2.24 \times 10^{-3}$  & $3.73 \times 10^{-4}$  \\ \hline
[133,151]                & 0.005303 & 0.005914   & $-1.44 \times 10^{-1}$ & $-8.01 \times 10^{-3}$ \\ \hline\hline
\end{tabular}
}
\caption{44}
\label{tabella_divisa}
\end{minipage} \vfill
\vspace{5mm}
\begin{minipage}{0.68\textwidth}
\centering
\includegraphics[width=\linewidth]{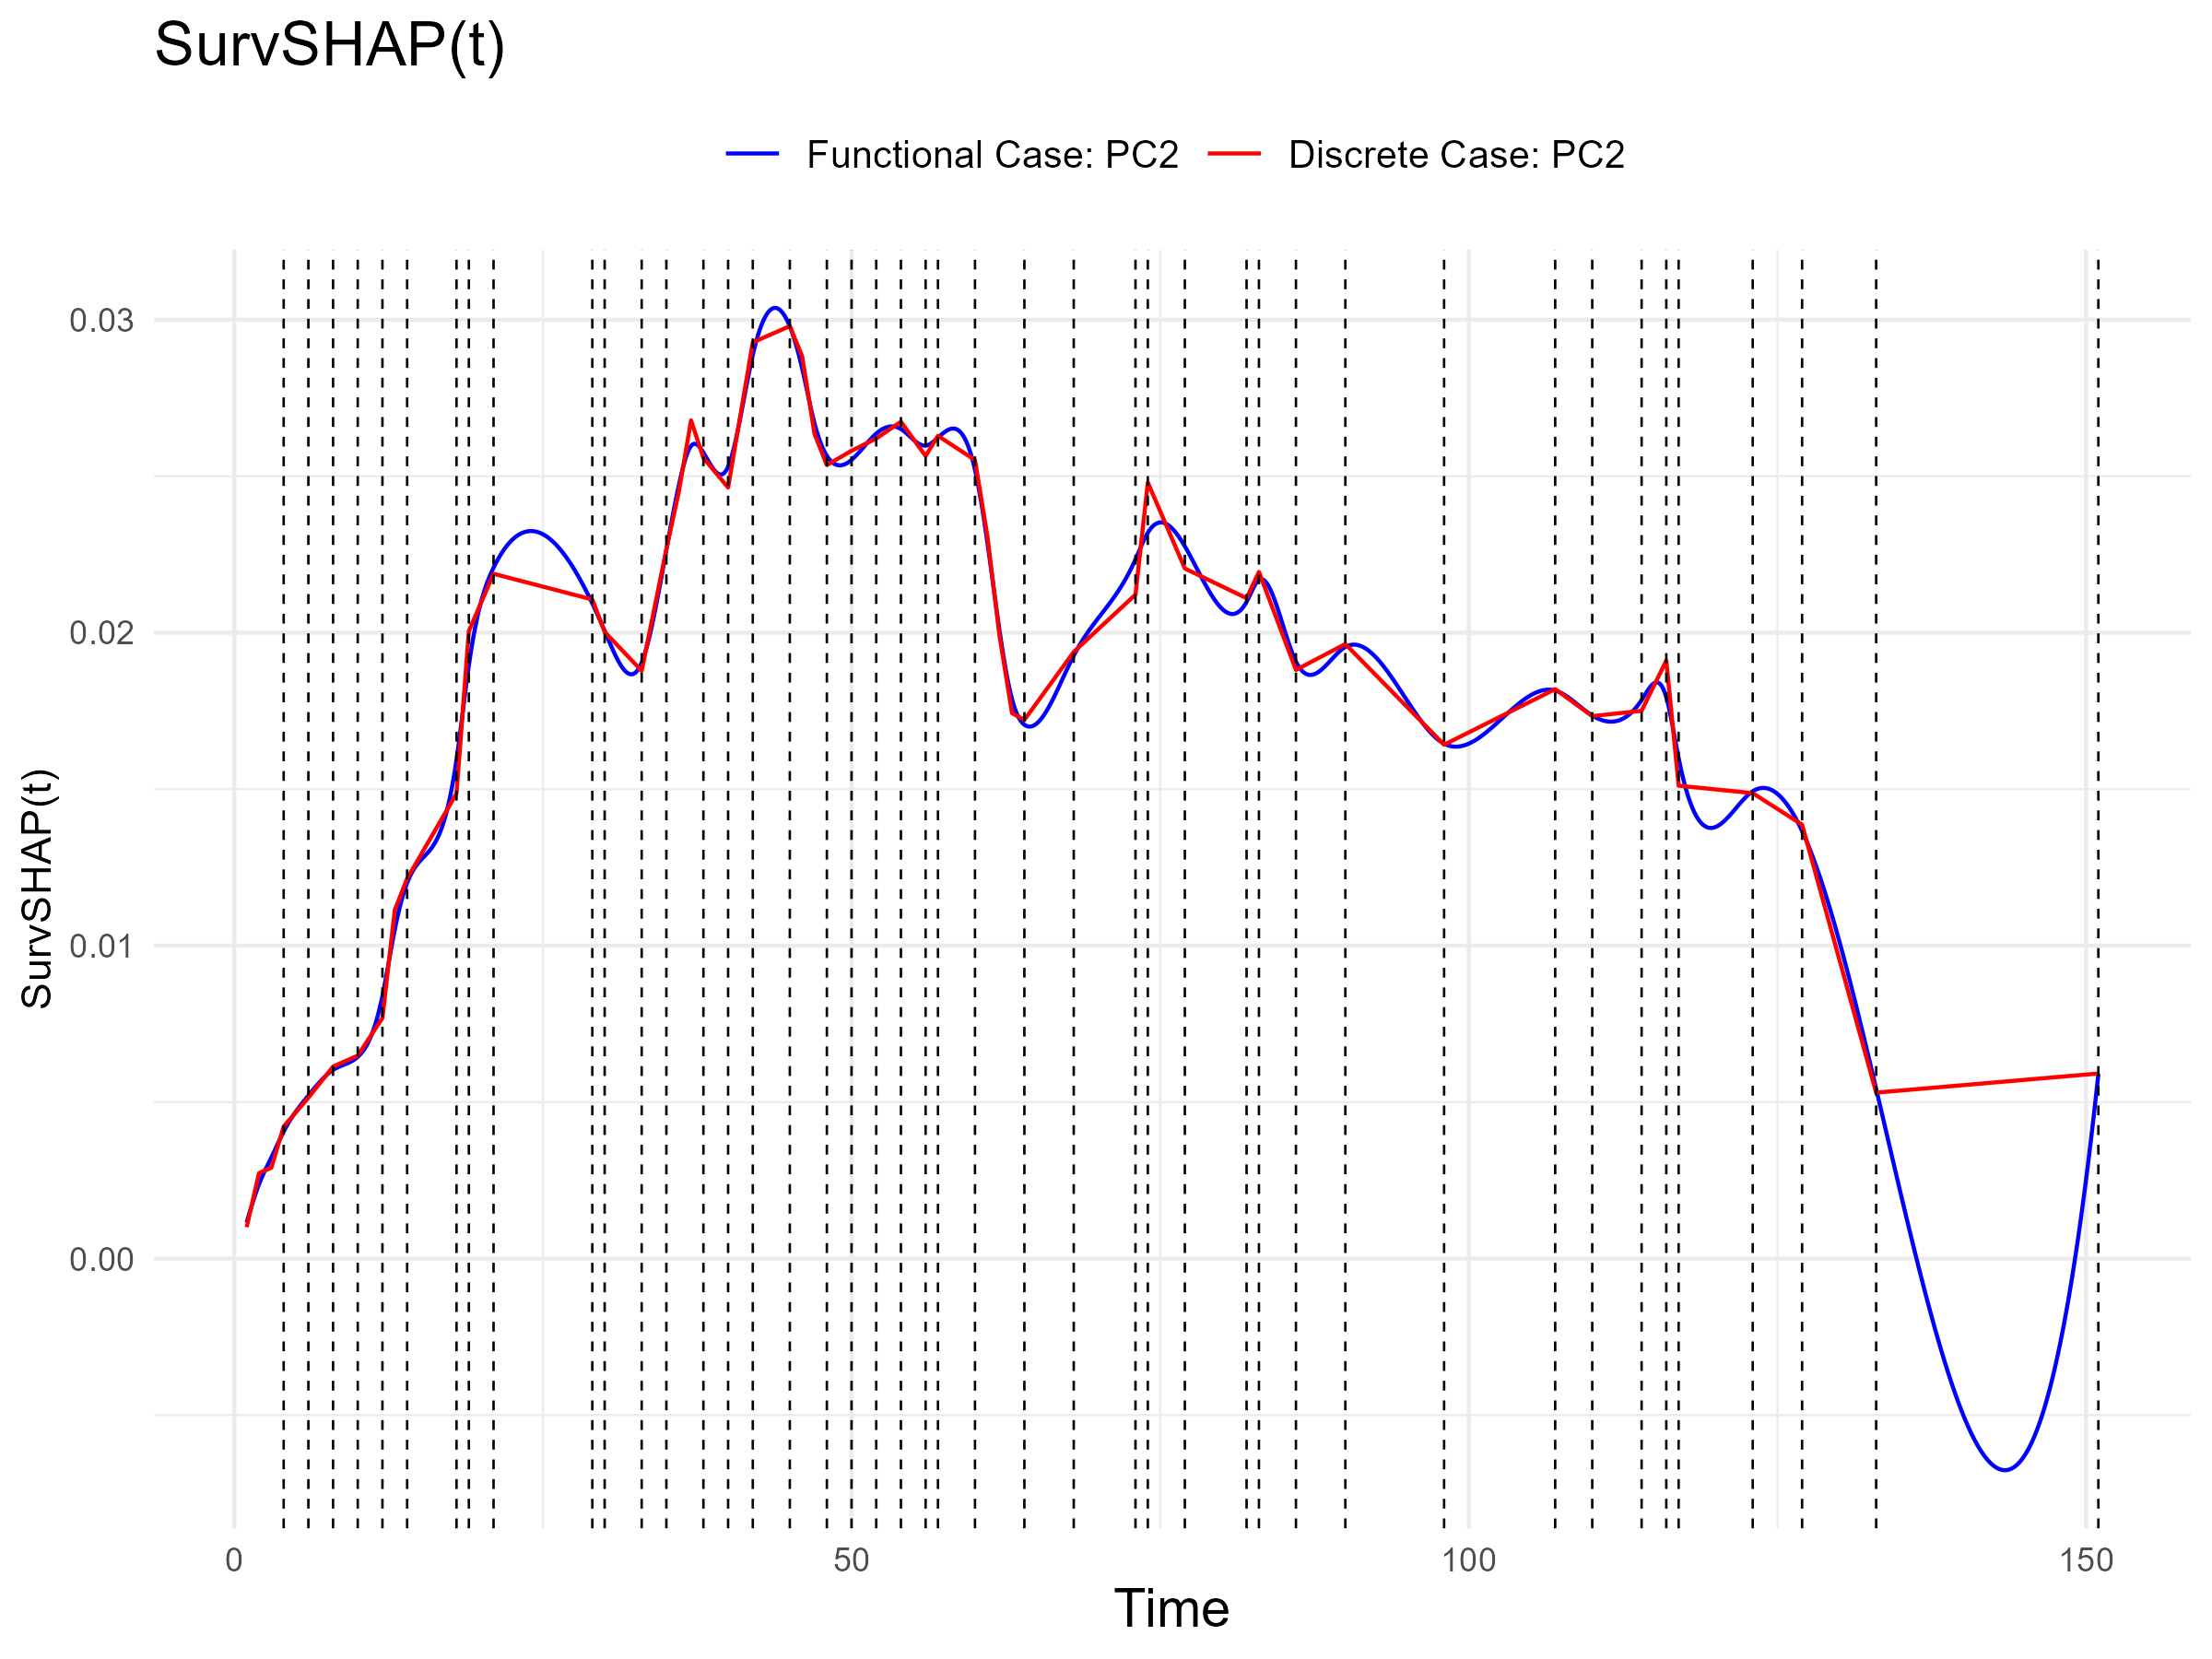}
\captionof{figure}{Descrizione dell'immagine.}
\label{fig:your_image}
\end{minipage}
\end{table*}

\newpage

\subsection*{Simulation study for $N=300$}

\begin{figure*}[h!]
    \centering
    \includegraphics[width=0.8\linewidth]{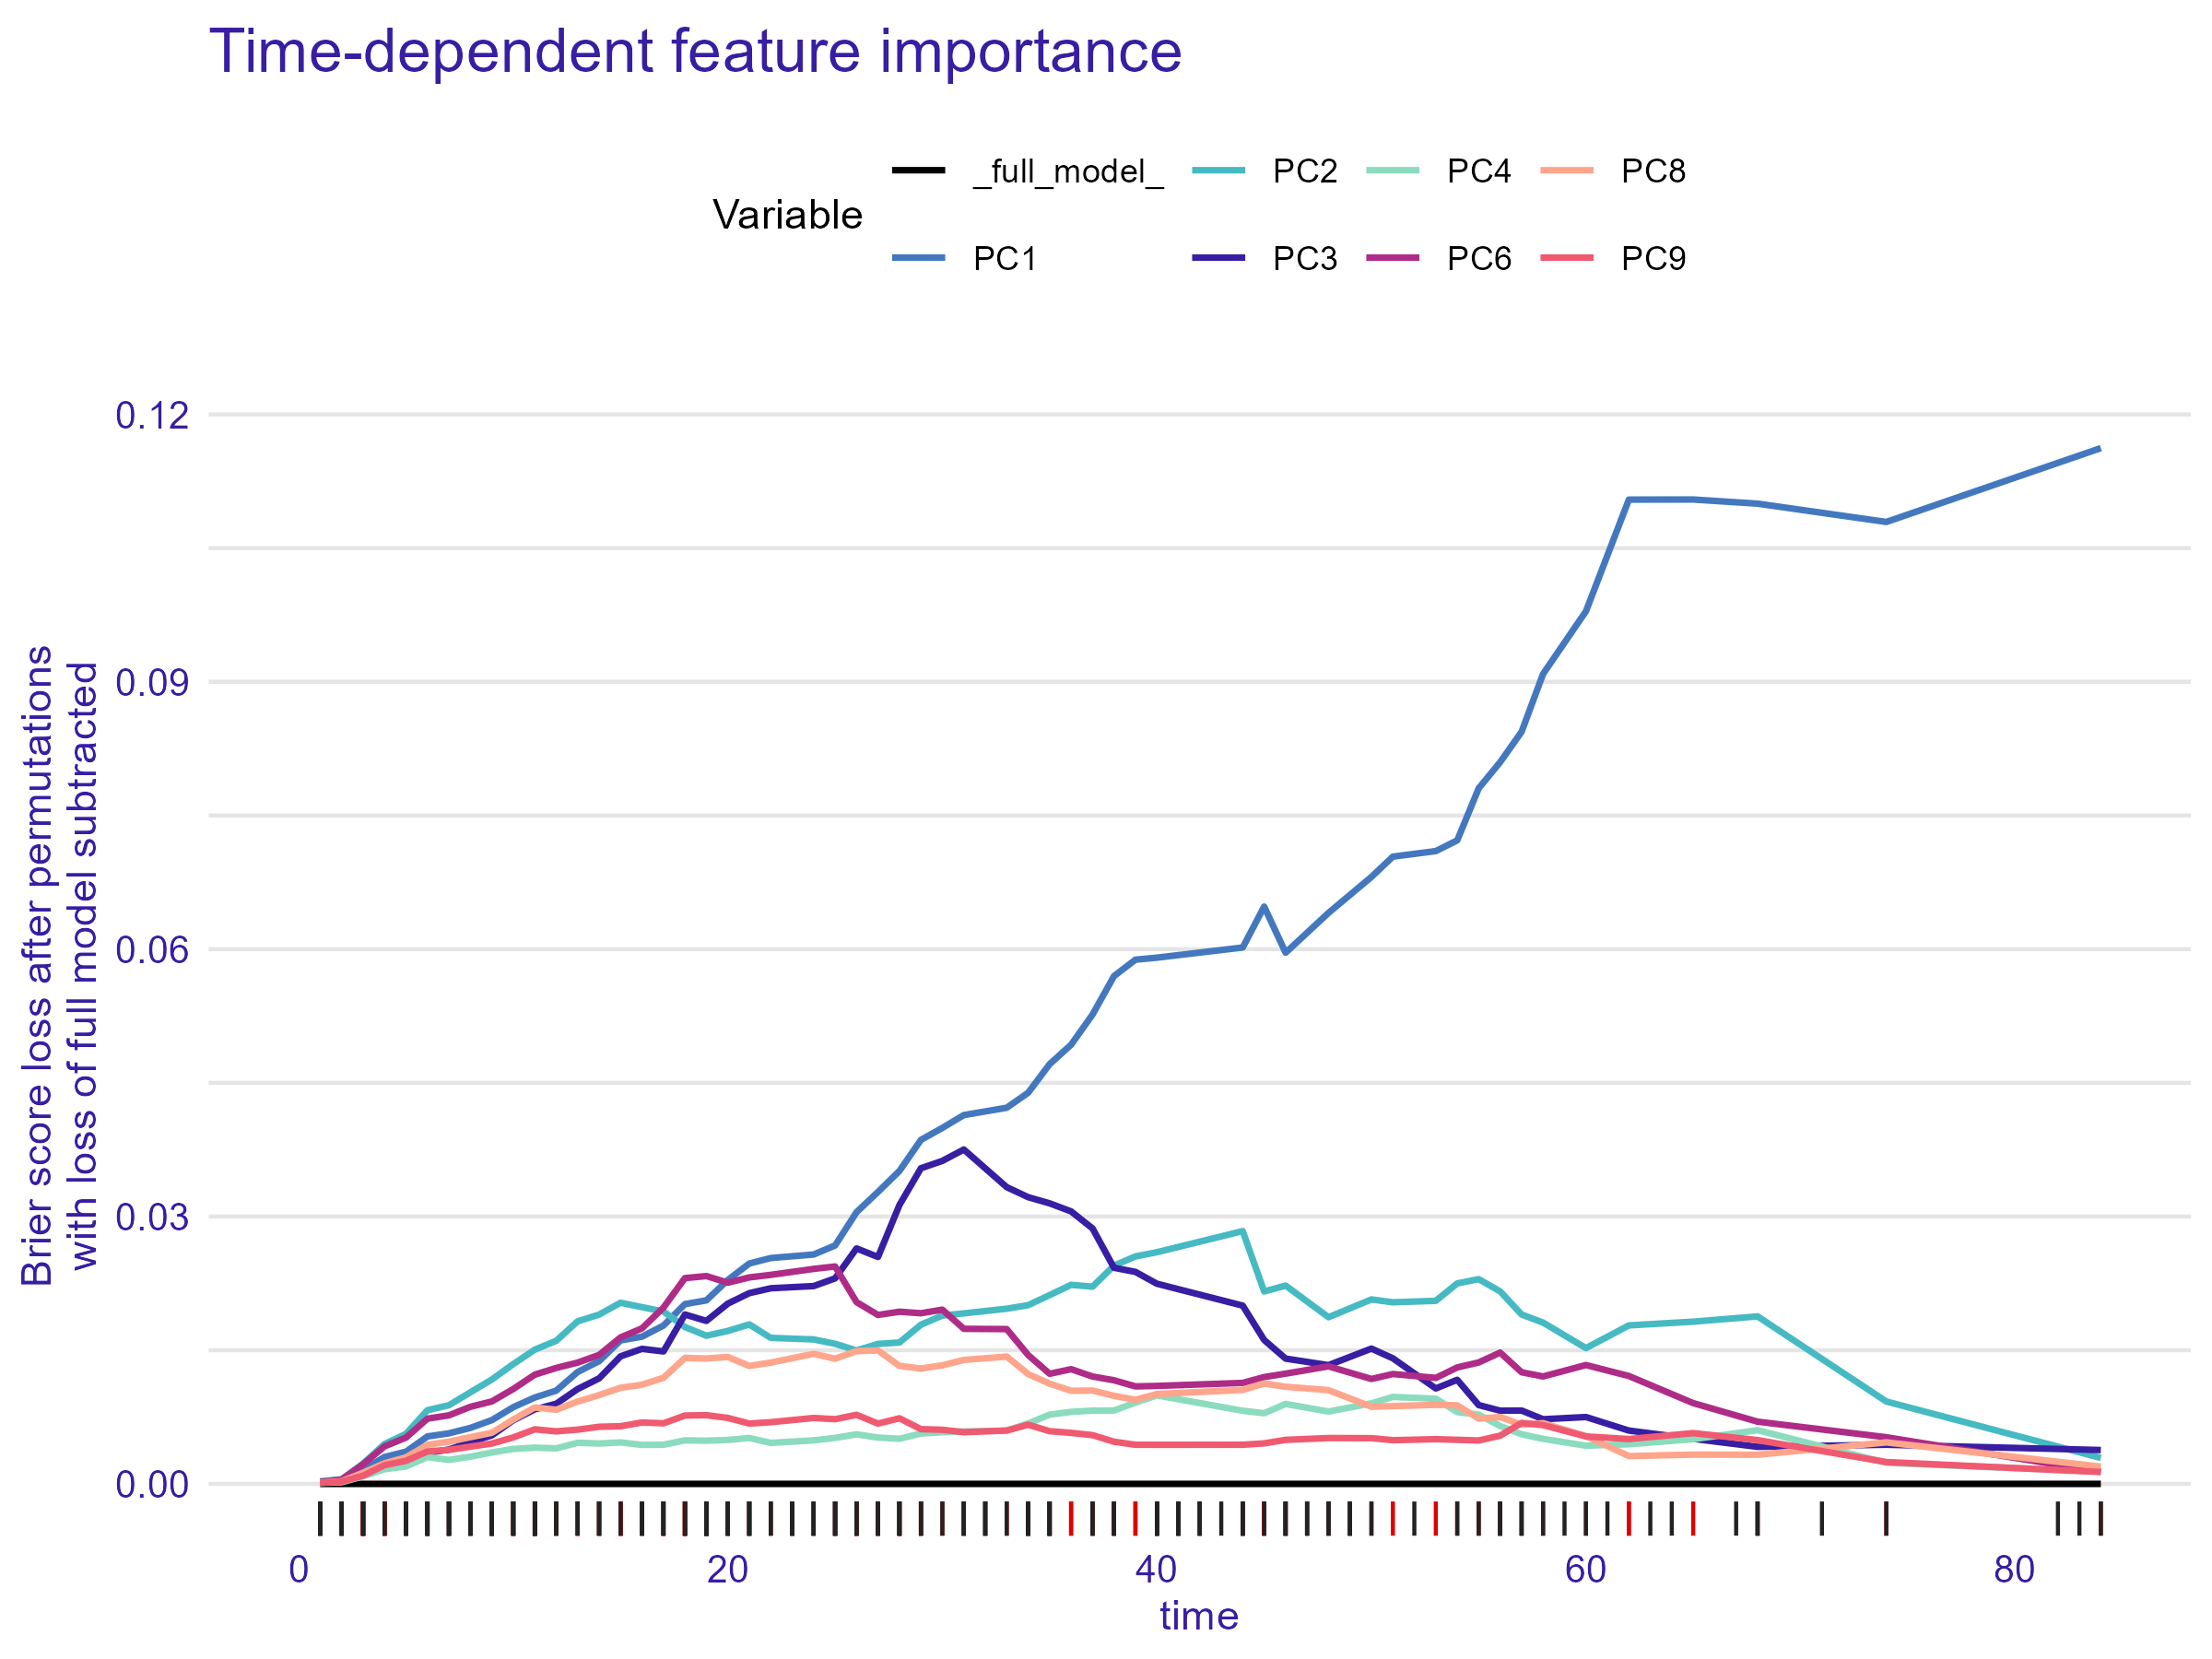}
    \includegraphics[width=0.8\linewidth]{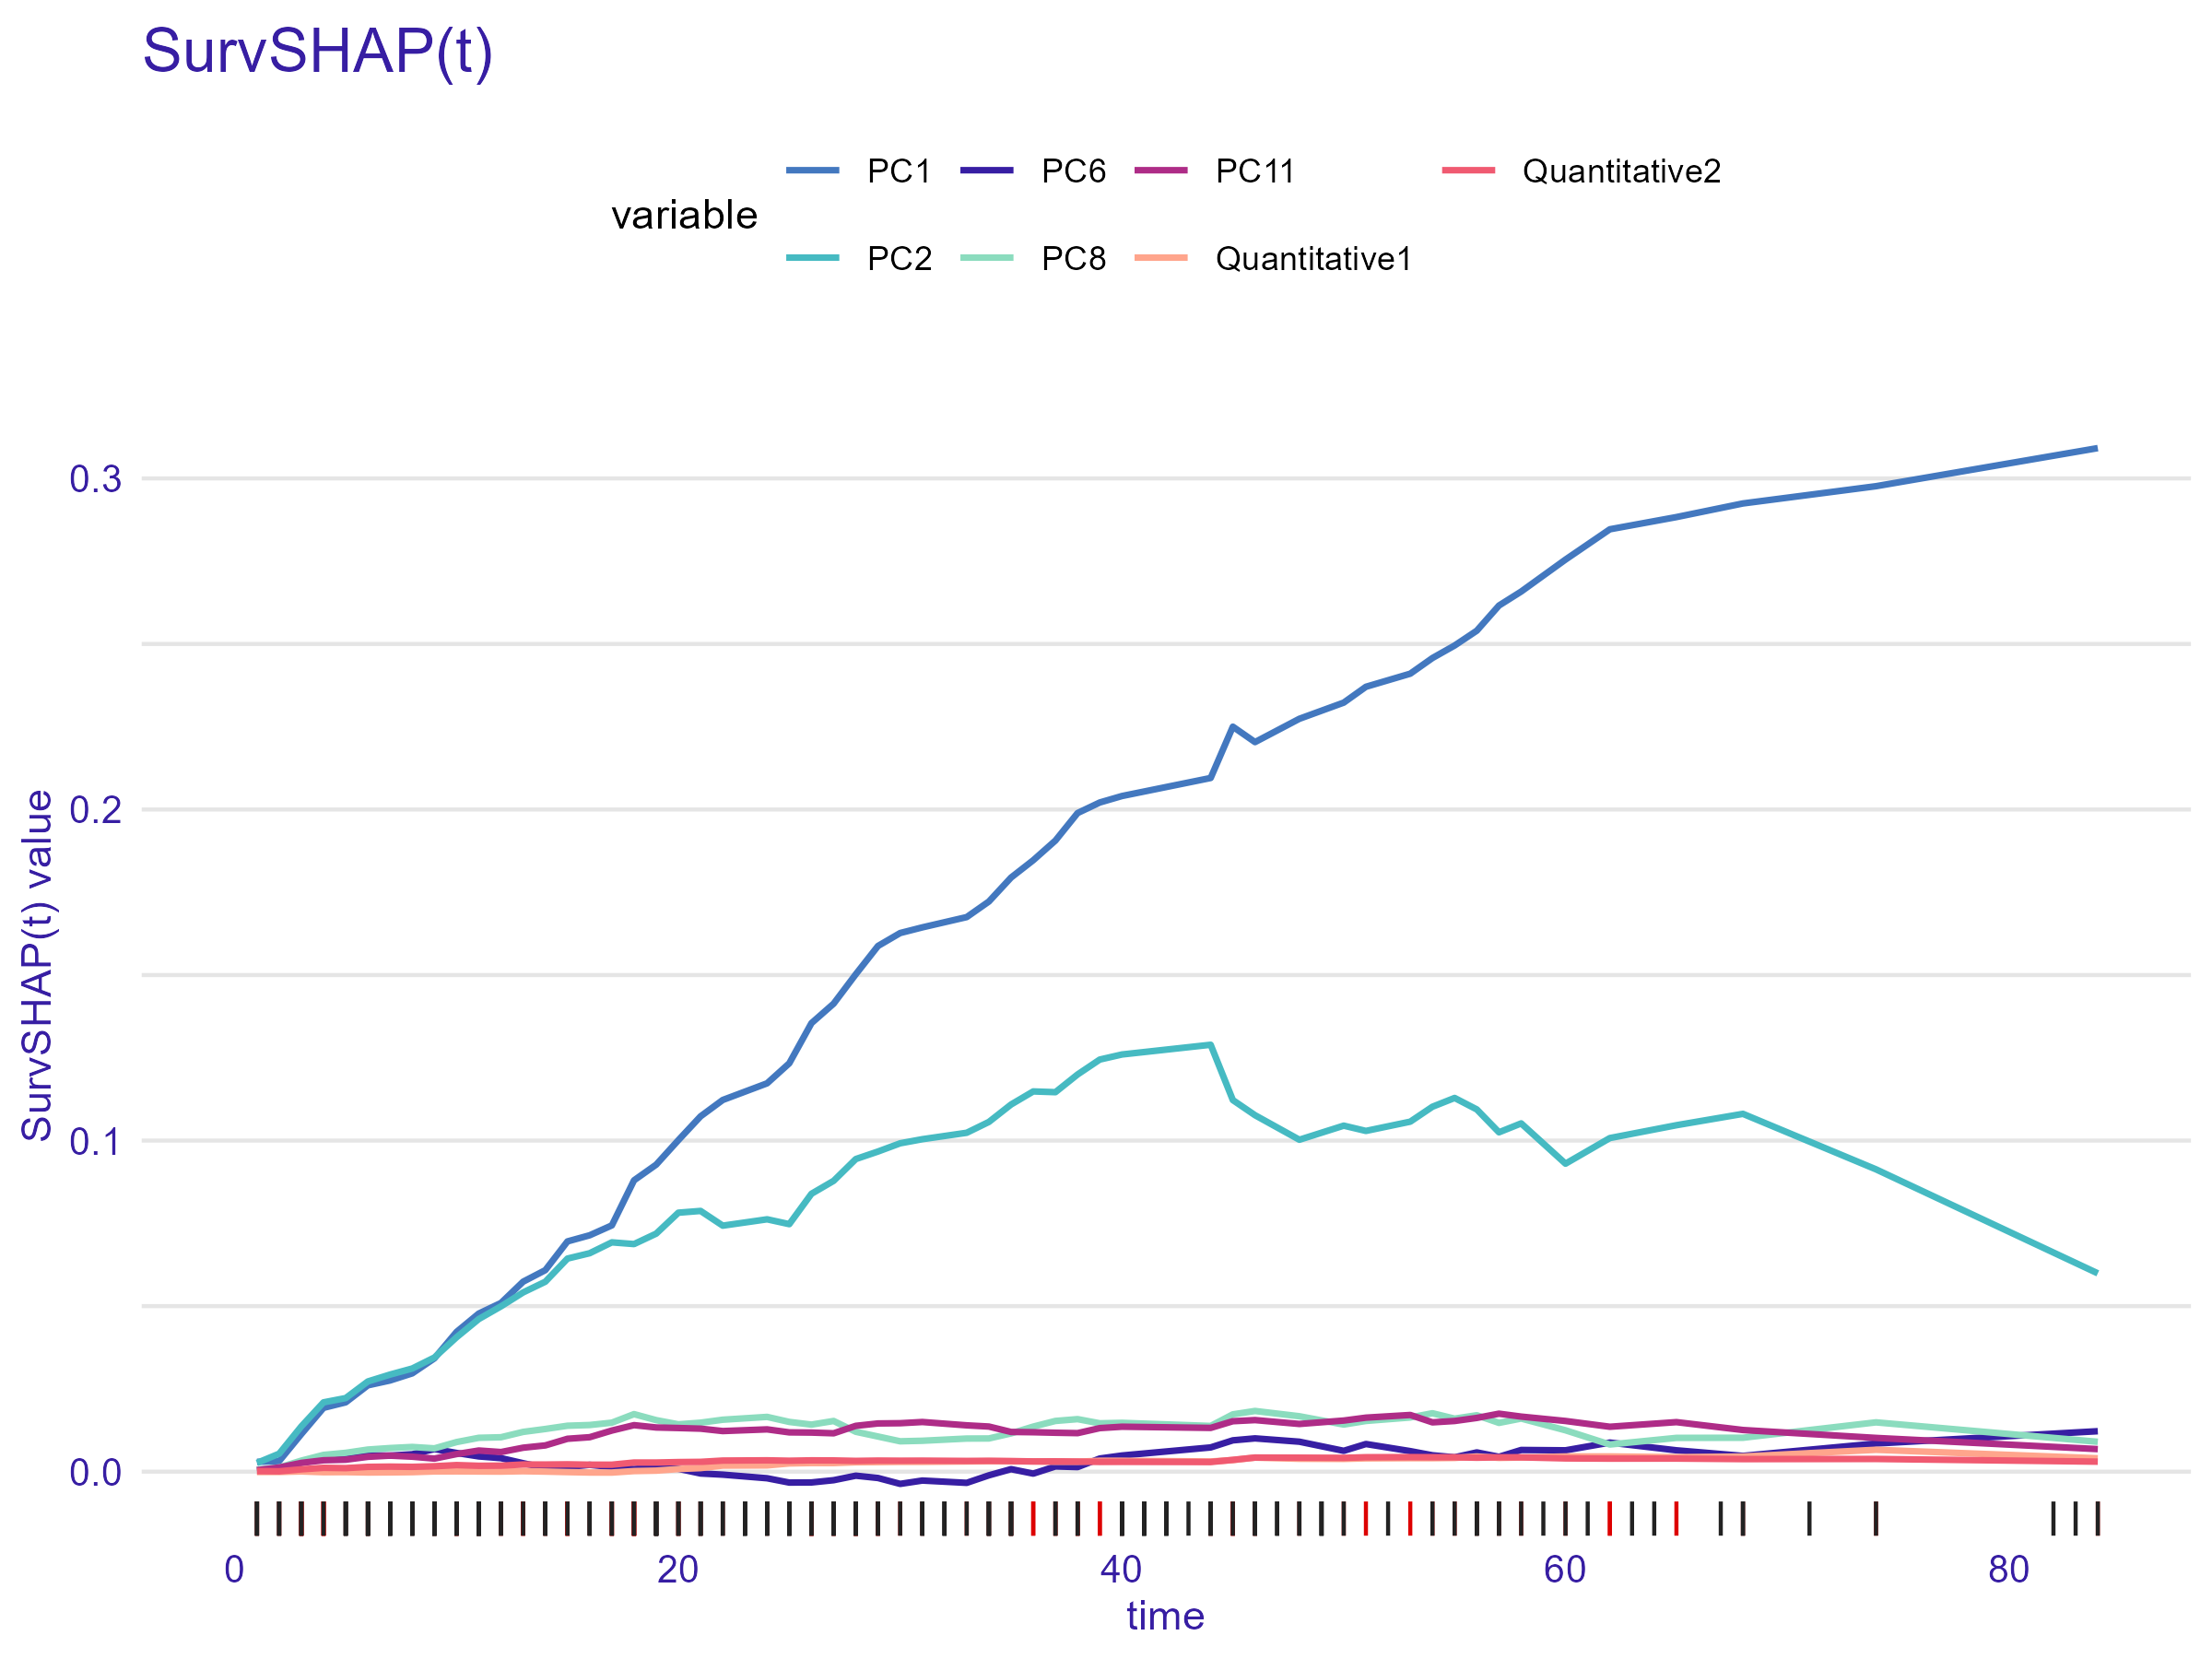}
    \caption{Caption}
    \label{fig:enter-label}
\end{figure*}

\begin{table*}
\Large
\centering
\begin{minipage}{0.70\textwidth}
\centering
 % Aumenta l'altezza delle righe
\setlength{\tabcolsep}{19pt} % Aumenta la spaziatura tra le colonne
\resizebox{\textwidth}{!}{ % Adatta la tabella alla larghezza della pagina
\begin{tabular}{c|cc|c|c} 
\hline
\hline
\multicolumn{5}{c}{\textbf{Global Explainability for PC1}} \\  
\hline
\hline
\multirow{2}{*}{\([t_\alpha,t_\beta]\)} & \multicolumn{2}{c|}{\(PFI_1(t)\)} & \multirow{2}{*}{\(MTSD_{t_\alpha,t_\beta}^{1}\)} &\multirow{2}{*} {\(MTNSD_{t_\alpha,t_\beta}^{1}\)} \\ \cline{2-3}
                        & \(PFI_1(t_\alpha)\) & \(PFI_1(t_\beta)\) &  &  \\ 
\hline
[22,24]                  & 0.025342 & 0.025739 & $7.02 \times 10^{-6}$   & $3.51 \times 10^{-6}$   \\ \hline
[31,33]                  & 0.041386 & 0.042205 & $-1.79 \times 10^{-4}$  & $-8.96 \times 10^{-5}$  \\ \hline
[40,44]                  & 0.059048 & 0.060188 & $-7.20 \times 10^{-3}$  & $-1.80 \times 10^{-3}$  \\ \hline
[46,48]                  & 0.059602 & 0.064075 & $-2.38 \times 10^{-3}$  & $-1.19 \times 10^{-3}$  \\ \hline
[48,50]                  & 0.064075 & 0.068107 & $1.02 \times 10^{-3}$   & $5.08 \times 10^{-4}$   \\ \hline
[51,53]                  & 0.070386 & 0.071006 & $1.70 \times 10^{-4}$   & $8.50 \times 10^{-5}$   \\ \hline
[58,60]                  & 0.090880 & 0.097922 & $1.21 \times 10^{-4}$   & $6.07 \times 10^{-5}$   \\ \hline
[60,62]                  & 0.097922 & 0.110446 & $2.09 \times 10^{-4}$   & $1.04 \times 10^{-4}$   \\ \hline
[62,65]                  & 0.110446 & 0.110457 & $4.14 \times 10^{-3}$   & $1.38 \times 10^{-3}$   \\ \hline
[65,68]                  & 0.110457 & 0.109992 & $-1.01 \times 10^{-3}$  & $-3.37 \times 10^{-4}$  \\ \hline
[68,74]                  & 0.109992 & 0.107939 & $1.89 \times 10^{-3}$   & $3.15 \times 10^{-4}$   \\ \hline
[74,84]                  & 0.107939 & 0.116225 & $-2.99 \times 10^{-2}$  & $-2.99 \times 10^{-3}$  \\ \hline \hline
\end{tabular}
}
\caption{44}
\label{tabella_divisa}
\end{minipage} \vfill
\vspace{5mm}
\begin{minipage}{0.68\textwidth}
\centering
\includegraphics[width=\linewidth]{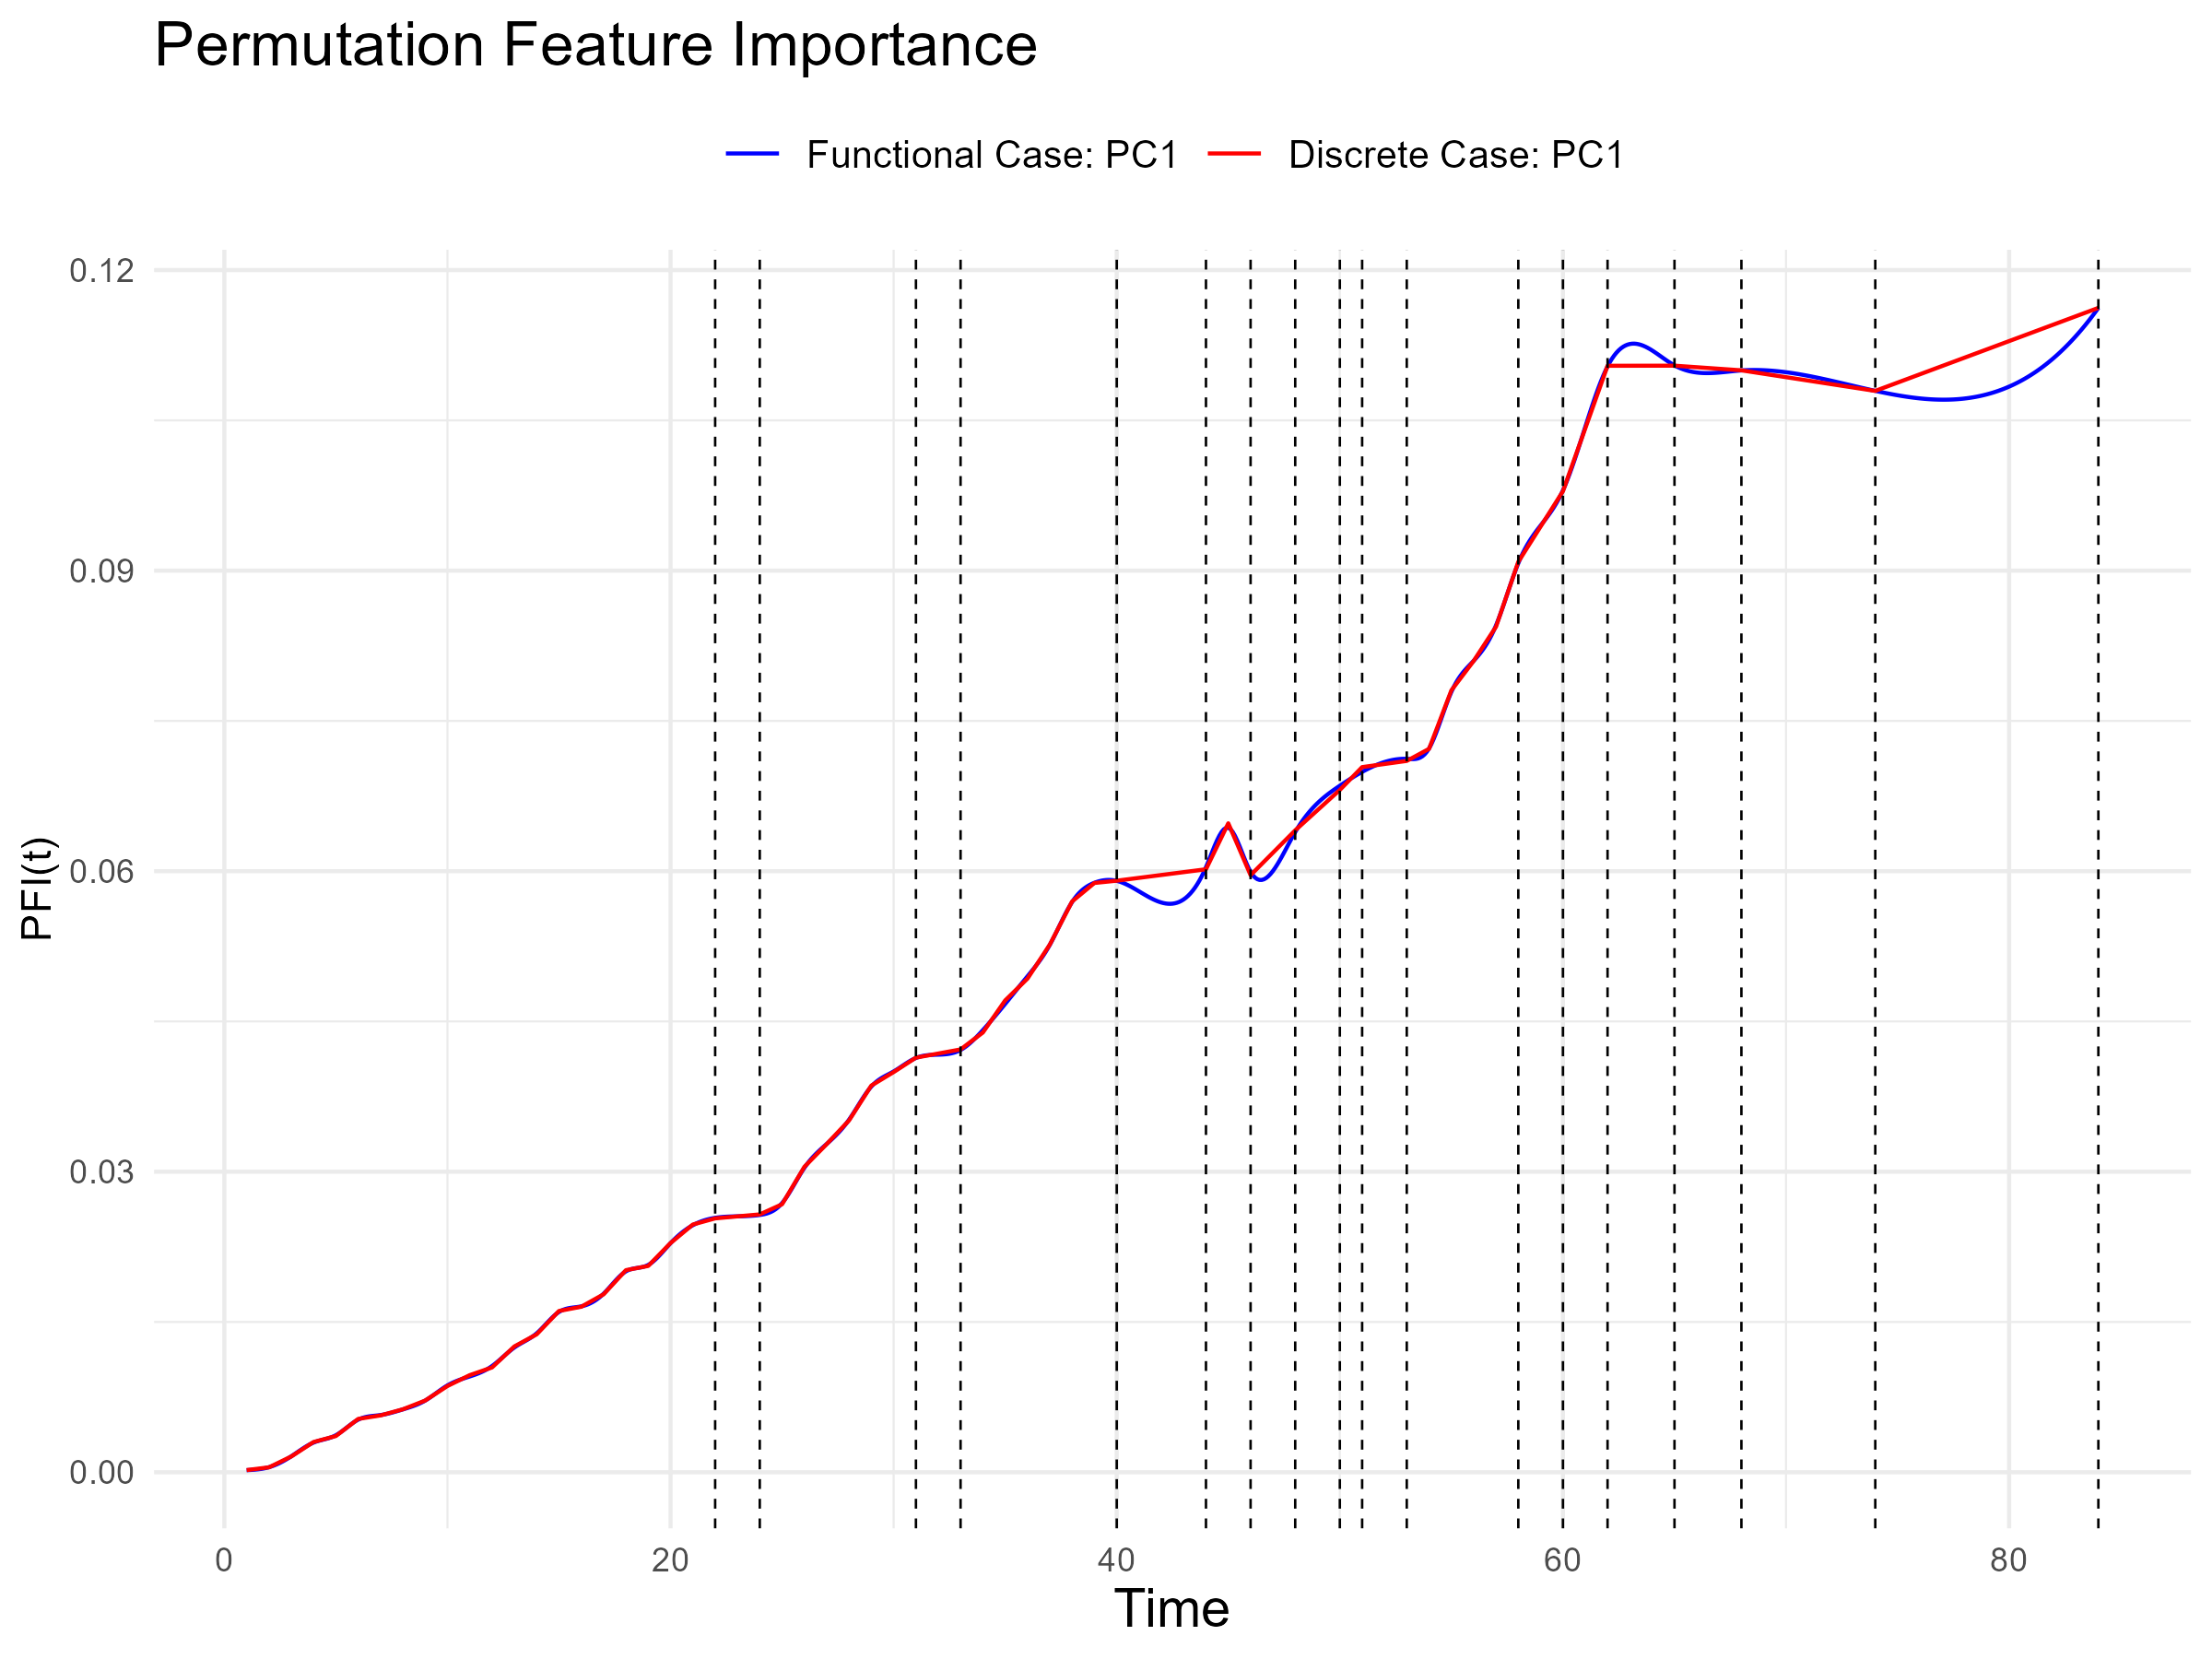}
\captionof{figure}{Descrizione dell'immagine.}
\label{fig:your_image}
\end{minipage}
\end{table*}  

\begin{table*}
\Large
\centering
\begin{minipage}{0.70\textwidth}
\centering
 % Aumenta l'altezza delle righe
\setlength{\tabcolsep}{19pt} % Aumenta la spaziatura tra le colonne
\resizebox{\textwidth}{!}{ % Adatta la tabella alla larghezza della pagina
\begin{tabular}{c|cc|c|c} 
\hline
\hline
\multicolumn{5}{c}{\textbf{Local Explainability for PC2 for $3$th unit}} \\  
\hline
\hline
\multirow{2}{*}{\([t_\alpha,t_\beta]\)} & \multicolumn{2}{c|}{\(\phi^*_t(\bm{w_*},2)\)} & \multirow{2}{*}{\(TSD_{t_\alpha,t_\beta}^{32}\)} &\multirow{2}{*} {\(TNSD_{t_\alpha,t_\beta}^{32}\)} \\ \cline{2-3}
                        & \(\phi^*_{t_\alpha}(\bm{w_*},2)\) & \(\phi^*_{t_\beta}(\bm{w_*},2)\) &  &  \\ 
\hline
[22,24]                    & 0.074305 & 0.076221 & $2.53 \times 10^{-6}$  & $1.27 \times 10^{-6}$  \\ \hline
[31,33]                    & 0.100418 & 0.102359 & $-5.05 \times 10^{-4}$ & $-2.53 \times 10^{-4}$ \\ \hline
[40,44]                    & 0.126007 & 0.128943 & $1.86 \times 10^{-2}$  & $4.65 \times 10^{-3}$  \\ \hline
[46,48]                    & 0.107663 & 0.100255 & $-1.78 \times 10^{-3}$ & $-8.90 \times 10^{-4}$ \\ \hline
[48,50]                    & 0.100255 & 0.104507 & $-1.01 \times 10^{-3}$ & $-5.06 \times 10^{-4}$ \\ \hline
[51,53]                    & 0.102917 & 0.105715 & $-5.80 \times 10^{-4}$ & $-2.90 \times 10^{-4}$ \\ \hline
[58,60]                    & 0.105192 & 0.093024 & $-5.87 \times 10^{-4}$ & $-2.93 \times 10^{-4}$ \\ \hline
[60,62]                    & 0.093024 & 0.100763 & $-1.68 \times 10^{-3}$ & $-8.39 \times 10^{-4}$ \\ \hline
[62,65]                    & 0.100763 & 0.104643 & $2.26 \times 10^{-3}$  & $7.53 \times 10^{-4}$  \\ \hline
[65,68]                    & 0.104643 & 0.108075 & $5.04 \times 10^{-4}$  & $1.68 \times 10^{-4}$  \\ \hline
[68,74]                    & 0.108075 & 0.091310 & $1.44 \times 10^{-2}$  & $2.40 \times 10^{-3}$  \\ \hline
[74,84]                    & 0.091310 & 0.059902 & $-4.97 \times 10^{-2}$ & $-4.97 \times 10^{-3}$ \\ \hline\hline
\end{tabular}
}
\caption{44}
\label{tabella_divisa}
\end{minipage} \vfill
\vspace{5mm}
\begin{minipage}{0.68\textwidth}
\centering
\includegraphics[width=\linewidth]{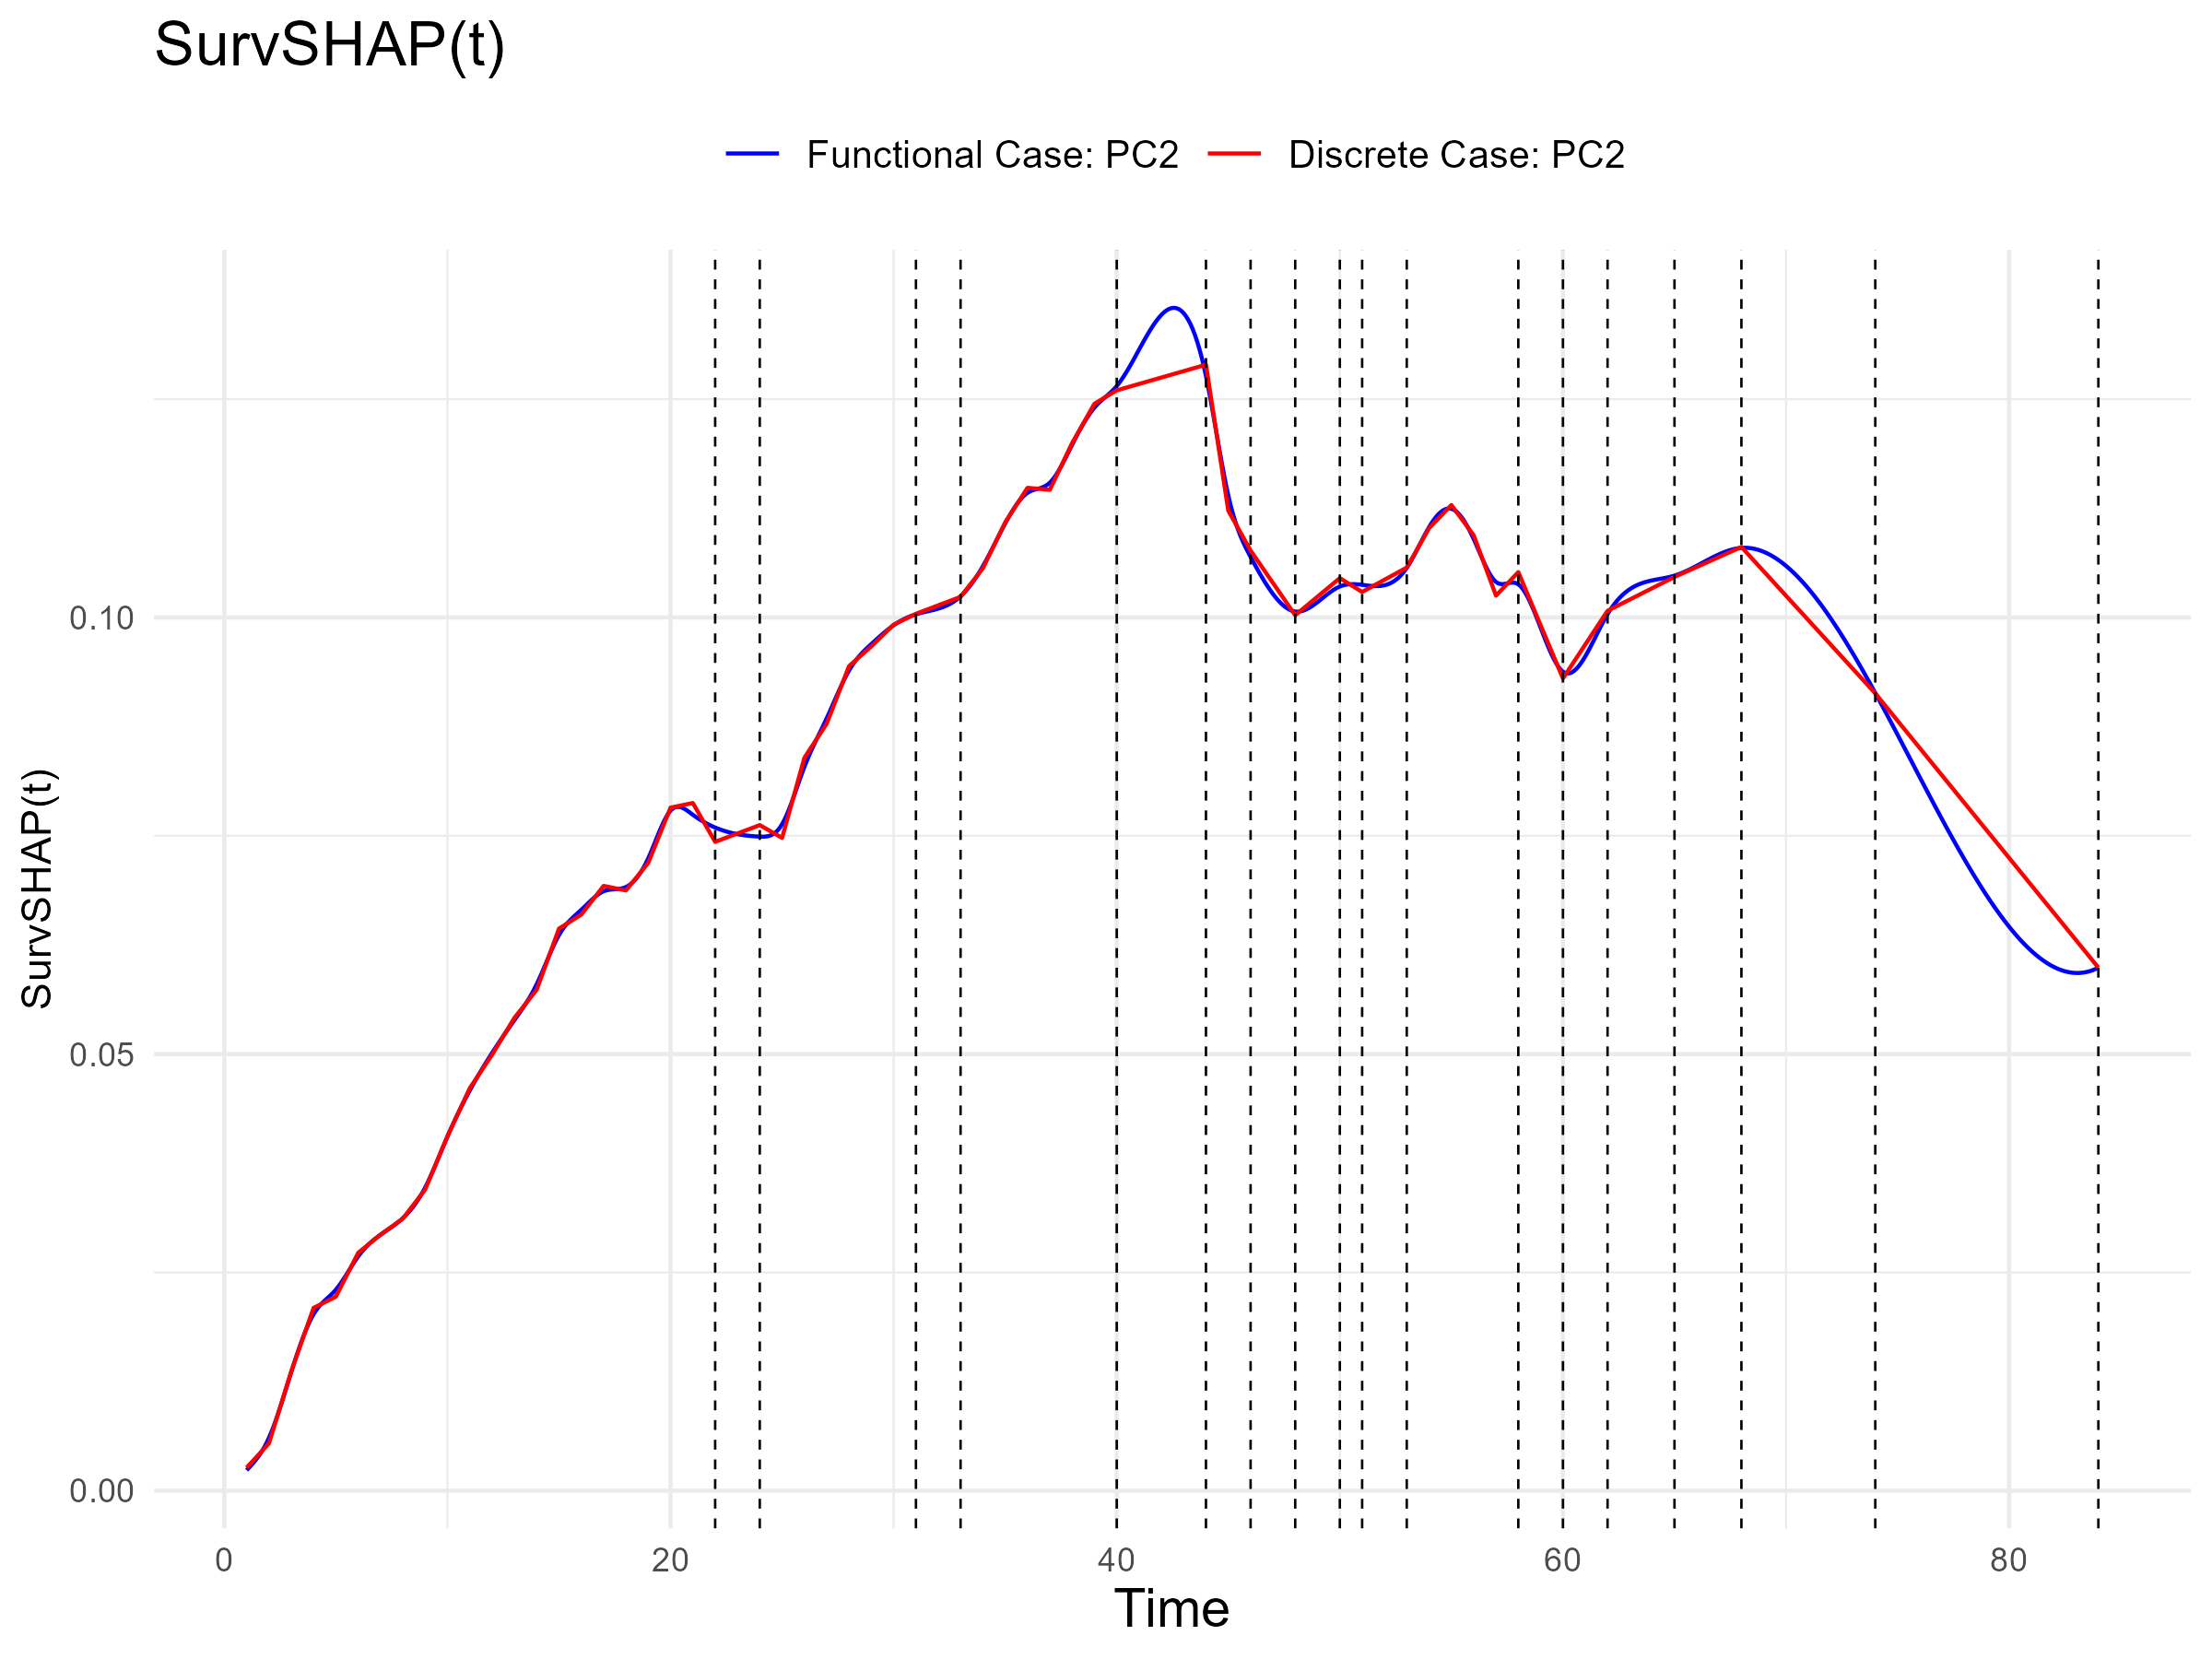}
\captionof{figure}{Descrizione dell'immagine.}
\label{fig:your_image}
\end{minipage}
\end{table*}

\newpage
